# Supplementary material for: A Cable Knot and BPS-Series
Source: arXiv:2101.11708 ancillary file (2023-01-18)
Supplement: Supplementary file 1 [file README.pdf]

# Additional documentation for “A Cable Knot and the BPS-Series”

John Chae

Department of Physics and QMAP, UC Davis, 1 Shields Ave, Davis, CA, 95616, USA  
yjchae@ucdavis.edu

This document is one of the three ancillary files that contains the details of the recursion relation in [1]. The other two documents contain the initial data for the  $f_m$ -recursion relation and the expressions for the coefficient functions  $t_v(q, q^m)$  in it, respectively.

## Definitions of the Coefficients in the Recursion Relation

We write the coefficient functions  $\alpha, \beta, \gamma, \delta$  of the recursion relation for the  $F_K$  (8) in Section 4 in [1].

$$\alpha(x, q) = \frac{N(\alpha)}{D(\alpha)},$$

$$\begin{aligned} D(\alpha) = & q^{66}x^{33} - q^{64}x^{31} + q^{63}x^9(x^{22} - x^{20}) + q^{62}x^9(-2x^{22} - x^{20}) - q^{61}x^{29} \\ & + q^{60}x^9(2x^{20} - x^{18}) + q^{59}x^9(-2x^{20} + 2x^{18} + x^{16}) + q^{58}x^9(x^{20} + x^{18}) \\ & + q^{57}x^9(-x^{20} + 2x^{18} + x^{16}) + q^{56}x^9(-2x^{18} + 2x^{16} + x^{14}) + q^{55}x^9(3x^{18} - x^{16} - x^{14}) \\ & + q^{54}x^9(-2x^{18} + 2x^{16} + x^{14} - x^{12}) + q^{53}x^9(x^{18} - x^{16} - x^{14} + x^{12}) \\ & + q^{52}x^9(3x^{16} - 2x^{14} - 2x^{12}) + q^{51}x^9(-2x^{16} + 2x^{14} - x^{10}) \\ & + q^{50}x^9(2x^{16} - 2x^{14} - 3x^{12} + 2x^{10}) + q^{49}x^9(x^{14} - 2x^{10}) + q^{48}x^9(x^{10} - 2x^{14}) \\ & + q^{47}x^9(2x^{14} - 3x^{12} - 2x^{10} + 2x^8) + q^{46}x^9(-x^{14} + 2x^{10} - 2x^8) \\ & + q^{45}x^9(-2x^{12} - 2x^{10} + 3x^8) + q^{44}x^9(x^{12} - x^{10} - x^8 + x^6) \\ & + q^{43}x^9(-x^{12} + x^{10} + 2x^8 - 2x^6) + q^{42}x^9(-x^{10} - x^8 + 3x^6) \\ & + q^{41}x^9(x^{10} + 2x^8 - 2x^6) + q^{40}x^9(x^8 + 2x^6 - x^4) + q^{39}x^9(x^6 + x^4) \\ & + q^{38}x^9(x^8 + 2x^6 - 2x^4) + q^{37}x^9(2x^4 - x^6) - q^{36}x^{13} + q^{35}x^9(-x^4 - 2x^2) \\ & + q^{34}x^9(x^2 - x^4) - q^{33}x^{11} + q^{31}x^9 \end{aligned}$$

$$\begin{aligned} N(\alpha) = & q^{61}(-x^{24}) + 2q^{57}x^{22} - q^{56}x^{22} + q^{55}x^{22} + q^{54}x^{20} - q^{53}x^{20} + 2q^{52}x^{20} - 2q^{51}x^{20} \\ & - q^{50}(x^{18} - x^{20}) - q^{49}(-x^{20} - 2x^{18}) - q^{48}(3x^{18} - x^{20}) + 2q^{47}x^{18} - 2q^{46}x^{18} \\ & - q^{45}(x^{18} + 2x^{16}) - q^{44}(2x^{18} - 2x^{16}) - q^{43}(3x^{16} - x^{18}) + q^{42}x^{16} \\ & - q^{41}(2x^{16} - x^{14}) - q^{40}(2x^{14} - x^{16}) - q^{39}(2x^{16} - 2x^{14}) - q^{38}(x^{16} + x^{14}) \\ & + 2q^{37}x^{14} - q^{36}(x^{16} + 2x^{14} - x^{12}) - q^{35}(x^{12} - 2x^{14}) - q^{34}(-x^{14} - 2x^{12}) \\ & - q^{33}x^{14} - q^{32}(-x^{14} - 3x^{12}) - q^{31}x^{14} - q^{30}x^{10} - q^{29}(-3x^{12} - x^{10}) - q^{28}x^{10} \\ & - q^{27}(-2x^{12} - x^{10}) - q^{26}(x^{12} - 2x^{10}) - q^{25}(-x^{12} + 2x^{10} + x^8) + 2q^{24}x^{10} \\ & - q^{23}(x^{10} + x^8) - q^{22}(2x^8 - 2x^{10}) - q^{21}(2x^{10} - x^8) - q^{20}(2x^8 - x^{10}) \end{aligned}$$

$$\begin{aligned}
& + q^{19}x^8 - q^{18}(3x^8 - x^6) - q^{17}(2x^6 - 2x^8) - q^{16}(2x^8 + x^6) - 2q^{15}x^6 + 2q^{14}x^6 \\
& - q^{13}(3x^6 - x^4) - q^{12}(-2x^6 - x^4) - q^{11}(x^6 - x^4) - 2q^{10}x^4 + 2q^9x^4 - q^8x^4 + q^7x^4 \\
& + q^6x^2 - q^5x^2 + 2q^4x^2 - 1.
\end{aligned}$$

$$\beta(x, q) = \frac{N(\beta)}{D(\beta)},$$

$$\begin{aligned}
D(\beta) = & q^{159/2}x^{41} - q^{155/2}x^{39} - q^{149/2}x^{37} - q^{99/2}x^{21} - q^{93/2}x^{19} + q^{89/2}x^{17} + q^{153/2}x^{17}(x^{22} - x^{20}) \\
& + q^{151/2}x^{17}(-2x^{22} - x^{20}) + q^{147/2}x^{17}(2x^{20} - x^{18}) + q^{143/2}x^{17}(x^{20} + x^{18}) \\
& + q^{125/2}x^{17}(x^{14} - 2x^{10}) + q^{123/2}x^{17}(x^{10} - 2x^{14}) + q^{105/2}x^{17}(x^6 + x^4) \\
& + q^{101/2}x^{17}(2x^4 - x^6) + q^{97/2}x^{17}(-x^4 - 2x^2) + q^{95/2}x^{17}(x^2 - x^4) \\
& + q^{145/2}x^{17}(-2x^{20} + 2x^{18} + x^{16}) + q^{141/2}x^{17}(-x^{20} + 2x^{18} + x^{16}) \\
& + q^{139/2}x^{17}(-2x^{18} + 2x^{16} + x^{14}) + q^{137/2}x^{17}(3x^{18} - x^{16} - x^{14}) \\
& + q^{131/2}x^{17}(3x^{16} - 2x^{14} - 2x^{12}) + q^{129/2}x^{17}(-2x^{16} + 2x^{14} - x^{10}) \\
& + q^{119/2}x^{17}(-x^{14} + 2x^{10} - 2x^8) + q^{117/2}x^{17}(-2x^{12} - 2x^{10} + 3x^8) \\
& + q^{111/2}x^{17}(-x^{10} - x^8 + 3x^6) + q^{109/2}x^{17}(x^{10} + 2x^8 - 2x^6) + q^{107/2}x^{17}(x^8 + 2x^6 - x^4) \\
& + q^{103/2}x^{17}(x^8 + 2x^6 - 2x^4) + q^{135/2}x^{17}(-2x^{18} + 2x^{16} + x^{14} - x^{12}) \\
& + q^{133/2}x^{17}(x^{18} - x^{16} - x^{14} + x^{12}) + q^{127/2}x^{17}(2x^{16} - 2x^{14} - 3x^{12} + 2x^{10}) \\
& + q^{121/2}x^{17}(2x^{14} - 3x^{12} - 2x^{10} + 2x^8) + q^{115/2}x^{17}(x^{12} - x^{10} - x^8 + x^6) \\
& + q^{113/2}x^{17}(-x^{12} + x^{10} + 2x^8 - 2x^6)
\end{aligned}$$

$$\begin{aligned}
N(\beta) = & -(x^{41} - x^{40})q^{79} - x^{38}q^{77} - (x^{38} + x^{36})q^{76} - (-2x^{39} + 2x^{38} + x^{36})q^{75} - (x^{39} - x^{38})q^{74} \\
& - (-x^{39} + x^{38} - x^{36} - x^{34})q^{73} - (-x^{37} - 3x^{34} - x^{32})q^{72} - (x^{37} - x^{36} - 2x^{34} - x^{32})q^{71} \\
& - (-2x^{37} + x^{36} - x^{34} - 2x^{32})q^{70} - (2x^{37} - 2x^{36} - 2x^{34})q^{69} \\
& - (-x^{37} + x^{36} + x^{35} - x^{34} + 2x^{30})q^{68} - (-x^{37} + x^{36} - 2x^{35} + x^{34} + x^{30} + x^{28})q^{67} \\
& - (-x^{37} + x^{36} + 3x^{35} - 2x^{34} + 4x^{30} + x^{28})q^{66} - (-2x^{35} + x^{32} + x^{30} + 2x^{28})q^{65} \\
& - (2x^{35} - 4x^{34} - 2x^{32} + 3x^{30} + x^{28})q^{64} \\
& - (x^{35} - 2x^{34} + 2x^{33} - 3x^{32} + x^{30} + 3x^{28} - x^{26})q^{63} \\
& - (2x^{35} - 2x^{34} - 2x^{33} + 3x^{30} - x^{28})q^{62} \\
& - (-x^{35} + x^{34} + 3x^{33} - x^{32} + 2x^{30} + 4x^{28} - 2x^{26} - x^{24})q^{61} \\
& - (-x^{33} + 3x^{32} + 7x^{30} + x^{28} - x^{24})q^{60} \\
& - (2x^{33} - x^{32} - x^{31} + 7x^{30} + 6x^{28} - 3x^{26} - x^{24})q^{59} \\
& - (-x^{33} + 2x^{31} + 3x^{30} + 3x^{28} + x^{26} - 2x^{24})q^{58} \\
& - (2x^{33} - 2x^{32} - 2x^{31} + 3x^{30} + 4x^{28} - 5x^{26} - x^{24} + x^{22})q^{57}
\end{aligned}$$

$$\begin{aligned}
& - (x^{33} - x^{32} + x^{31} + x^{30} - x^{28} - 2x^{26} - 4x^{24} - x^{22}) q^{56} \\
& - (-2x^{31} + 2x^{30} + x^{28} - 9x^{26} - 2x^{24}) q^{55} \\
& - (x^{33} - x^{32} + 2x^{31} + x^{30} - x^{29} + 2x^{28} - 4x^{26} - 8x^{24} + x^{22} + x^{20}) q^{54} \\
& - (-2x^{31} + 3x^{30} + x^{29} + 3x^{28} - 8x^{26} - 3x^{24} - x^{22}) q^{53} \\
& - (-x^{31} + 2x^{30} - 2x^{29} + 4x^{28} - x^{26} - 8x^{24} + x^{22} + 2x^{20}) q^{52} \\
& - (x^{31} + 3x^{28} - 3x^{26} - 2x^{24}) q^{51} \\
& - (-x^{31} + x^{30} - 3x^{29} + 3x^{28} - 4x^{26} - 7x^{24} + 5x^{22} + 2x^{20} - x^{18}) q^{50} \\
& - (x^{31} - x^{30} - 7x^{26} - 4x^{24} - x^{22} + 4x^{20} + 2x^{18}) q^{49} \\
& - (x^{28} + x^{27} - 5x^{26} - 11x^{24} + 4x^{22} + 3x^{20} - x^{18}) q^{48} \\
& - (-3x^{29} + 3x^{28} - x^{27} - 4x^{26} - 9x^{24} - 2x^{22} + 5x^{20} + x^{18}) q^{47} \\
& - (x^{28} + x^{27} - 3x^{26} - 7x^{24} + 3x^{22} + 3x^{20} - x^{18}) q^{46} \\
& - (-2x^{29} + 2x^{28} - x^{27} - 4x^{24} + x^{22} + 8x^{20} - 2x^{16}) q^{45} \\
& - (x^{29} - x^{28} - 2x^{27} - x^{26} - 5x^{24} + 7x^{22} + 6x^{20} + x^{18} + x^{16}) q^{44} \\
& - (-x^{29} + x^{28} + 2x^{27} - 3x^{26} + x^{25} - 6x^{24} + 6x^{22} + 11x^{20} + x^{18} - 2x^{16}) q^{43} \\
& - (-2x^{27} + x^{26} - 5x^{24} + 2x^{22} + 9x^{20} + 2x^{18}) q^{42} \\
& - (x^{27} - x^{26} + x^{25} - 5x^{24} + 11x^{20} - 3x^{16} + x^{14}) q^{41} \\
& - (-2x^{27} + x^{26} + 2x^{25} - 3x^{24} + 6x^{20} + 2x^{18} - 3x^{16} - 2x^{14}) q^{40} \\
& - (2x^{27} - 2x^{26} - x^{25} - 3x^{24} + 2x^{22} + 6x^{20} - 3x^{16} + x^{14}) q^{39} \\
& - (-x^{27} + x^{26} + 2x^{25} - 3x^{24} + 11x^{20} - 5x^{16} - x^{14}) q^{38} \\
& - (-x^{25} + 2x^{22} + 9x^{20} + 2x^{18} - 5x^{16} + x^{14}) q^{37} \\
& - (3x^{25} - 2x^{24} - x^{23} + x^{22} + 11x^{20} + 6x^{18} - 6x^{16} - 3x^{14} + x^{12}) q^{36} \\
& - (-2x^{25} + x^{24} + 2x^{23} + x^{22} + 6x^{20} + 7x^{18} - 5x^{16} - x^{14} - x^{12}) q^{35} \\
& - (2x^{25} - 2x^{24} + x^{23} + 8x^{20} + x^{18} - 4x^{16} + 2x^{12}) q^{34} \\
& - (2x^{23} - x^{22} + 3x^{20} + 3x^{18} - 7x^{16} - 3x^{14} + x^{12}) q^{33} \\
& - (-2x^{23} + x^{22} + 5x^{20} - 2x^{18} - 9x^{16} - 4x^{14} + 3x^{12}) q^{32} \\
& - (3x^{23} - x^{22} - x^{21} + 3x^{20} + 4x^{18} - 11x^{16} - 5x^{14} + x^{12}) q^{31} \\
& - (-2x^{23} + 2x^{22} - x^{21} + 4x^{20} - x^{18} - 4x^{16} - 7x^{14} - x^{10}) q^{30} \\
& - (x^{23} - x^{22} - x^{21} + 2x^{20} + 5x^{18} - 7x^{16} - 4x^{14} + 3x^{12} + x^{10}) q^{29} \\
& - (2x^{21} - 2x^{16} - 3x^{14} + 3x^{12}) q^{28} - (-2x^{21} + 2x^{20} + x^{18} - 8x^{16} - x^{14} + 4x^{12} + 2x^{10}) q^{27} \\
& - (x^{21} - x^{18} - 3x^{16} - 8x^{14} + 3x^{12} + 3x^{10}) q^{26} \\
& - (-x^{21} + x^{20} + x^{18} - 8x^{16} - 4x^{14} + 2x^{12} + x^{10} - x^8) q^{25} \\
& - (-x^{19} - 2x^{16} - 9x^{14} + x^{12} + 2x^{10}) q^{24} - (x^{19} - x^{18} - 4x^{16} - 2x^{14} - x^{12} + x^{10} - x^8) q^{23} \\
& - (-2x^{19} + x^{18} - x^{16} - 5x^{14} + 4x^{12} + 3x^{10} - 2x^8) q^{22} - (-2x^{16} + x^{14} + 3x^{12} + 3x^{10}) q^{21} \\
& - (-x^{16} - 3x^{14} + 6x^{12} + 7x^{10} - x^8) q^{20} - (-x^{16} + x^{12} + 7x^{10} + 3x^8) q^{19} \\
& - (x^{17} - x^{16} - 2x^{14} + 4x^{12} + 2x^{10} - x^8 + x^6) q^{18} - (-x^{12} + 3x^{10} - 2x^6) q^{17}
\end{aligned}$$

$$\begin{aligned}
& -(-x^{14} + 3x^{12} + x^{10} - 3x^8 - 2x^6)q^{16} - (x^{12} + 3x^{10} - 2x^8 - 4x^6)q^{15} \\
& - (2x^{12} + x^{10} + x^8)q^{14} - (x^{12} + 4x^{10} - 2x^6 + x^4)q^{13} - (x^{12} + x^{10} + x^6 + x^4)q^{12} \\
& - (2x^{10} - x^6 + x^4)q^{11} - (-2x^6 - 2x^4)q^{10} - (-2x^8 - x^6 + x^4)q^9 \\
& - (-x^8 - 2x^6 - x^4)q^8 - (-x^8 - 3x^6)q^7 - (-x^6 - x^4 + x^2)q^6 + x^2q^5 - (x^4 + 2x^2)q^4 \\
& - (x^4 + x^2)q^3 - x^2q^2 + 1.
\end{aligned}$$

$$\gamma(x, q) = \frac{N(\gamma)}{D(\gamma)},$$

$$\begin{aligned}
D(\gamma) = & q^{85}x^{41} - q^{83}x^{39} + q^{82}x^{17}(x^{22} - x^{20}) + q^{81}x^{17}(-2x^{22} - x^{20}) - q^{80}x^{37} \\
& + q^{79}x^{17}(2x^{20} - x^{18}) + q^{78}x^{17}(-2x^{20} + 2x^{18} + x^{16}) + q^{77}x^{17}(x^{20} + x^{18}) \\
& + q^{76}x^{17}(-x^{20} + 2x^{18} + x^{16}) + q^{75}x^{17}(-2x^{18} + 2x^{16} + x^{14}) \\
& + q^{74}x^{17}(3x^{18} - x^{16} - x^{14}) + q^{73}x^{17}(-2x^{18} + 2x^{16} + x^{14} - x^{12}) \\
& + q^{72}x^{17}(x^{18} - x^{16} - x^{14} + x^{12}) + q^{71}x^{17}(3x^{16} - 2x^{14} - 2x^{12}) \\
& + q^{70}x^{17}(-2x^{16} + 2x^{14} - x^{10}) + q^{69}x^{17}(2x^{16} - 2x^{14} - 3x^{12} + 2x^{10}) \\
& + q^{68}x^{17}(x^{14} - 2x^{10}) + q^{67}x^{17}(x^{10} - 2x^{14}) \\
& + q^{66}x^{17}(2x^{14} - 3x^{12} - 2x^{10} + 2x^8) + q^{65}x^{17}(-x^{14} + 2x^{10} - 2x^8) \\
& + q^{64}x^{17}(-2x^{12} - 2x^{10} + 3x^8) + q^{63}x^{17}(x^{12} - x^{10} - x^8 + x^6) \\
& + q^{62}x^{17}(-x^{12} + x^{10} + 2x^8 - 2x^6) + q^{61}x^{17}(-x^{10} - x^8 + 3x^6) \\
& + q^{60}x^{17}(x^{10} + 2x^8 - 2x^6) + q^{59}x^{17}(x^8 + 2x^6 - x^4) + q^{58}x^{17}(x^6 + x^4) \\
& + q^{57}x^{17}(x^8 + 2x^6 - 2x^4) + q^{56}x^{17}(2x^4 - x^6) - q^{55}x^{21} \\
& + q^{54}x^{17}(-x^4 - 2x^2) + q^{53}x^{17}(x^2 - x^4) - q^{52}x^{19} + q^{50}x^{17}
\end{aligned}$$

$$\begin{aligned}
N(\gamma) = & x^{49}q^{98} - x^{47}q^{96} + (-x^{47} - x^{45})q^{95} + (-2x^{47} - x^{45})q^{94} + x^{47}q^{93} \\
& + (-x^{47} + x^{45} + x^{43})q^{92} + (3x^{43} + x^{41})q^{91} + (x^{45} + 2x^{43} + x^{41})q^{90} \\
& + (-x^{45} + x^{43} + 2x^{41})q^{89} + (2x^{45} + 2x^{43})q^{88} + (-x^{45} + x^{43} - 2x^{39})q^{87} \\
& + (-x^{45} - x^{43} - x^{39} - x^{37})q^{86} + (-x^{45} + 2x^{43} - 4x^{39} - x^{37})q^{85} \\
& + (-x^{41} - x^{39} - 2x^{37})q^{84} + (4x^{43} + 2x^{41} - 3x^{39} - x^{37})q^{83} \\
& + (2x^{43} + 3x^{41} - x^{39} - 3x^{37} + x^{35})q^{82} + (2x^{43} - x^{40} - 3x^{39} + x^{37})q^{81} \\
& + (-x^{43} + x^{41} - 2x^{39} - 4x^{37} + 2x^{35} + x^{33})q^{80} + (-3x^{41} - 7x^{39} + x^{38} - x^{37} + x^{33})q^{79} \\
& + (x^{41} - 7x^{39} - x^{38} - 6x^{37} + x^{36} + 3x^{35} + x^{33})q^{78} \\
& + (-3x^{39} + 2x^{38} - 3x^{37} + x^{36} - x^{35} + 2x^{33})q^{77} \\
& + (2x^{41} - 3x^{39} + x^{38} - 4x^{37} + x^{36} + 5x^{35} + x^{33} - x^{31})q^{76} \\
& + (x^{41} - x^{39} + x^{38} + x^{37} - 2x^{36} + 2x^{35} + x^{34} + 4x^{33} + x^{31})q^{75}
\end{aligned}$$

$$\begin{aligned}
& + (-2x^{39} - x^{37} + x^{36} + 9x^{35} - 2x^{34} + 2x^{33} - x^{32}) q^{74} \\
& + (x^{41} - x^{39} - 2x^{37} - x^{36} + 4x^{35} - 2x^{34} + 8x^{33} - x^{31} - x^{29}) q^{73} \\
& + (-3x^{39} - 3x^{37} + 8x^{35} - 4x^{34} + 3x^{33} - x^{32} + x^{31}) q^{72} \\
& + (-2x^{39} - 4x^{37} - x^{36} + x^{35} + 8x^{33} - 2x^{32} - x^{31} - x^{30} - 2x^{29}) q^{71} \\
& + (-3x^{37} + 3x^{35} - 2x^{34} + 2x^{33} + x^{30}) q^{70} \\
& + (-x^{39} - 3x^{37} + x^{36} + 4x^{35} + x^{34} + 7x^{33} - x^{32} - 5x^{31} - 2x^{29} + x^{28} + x^{27}) q^{69} \\
& + (x^{39} + x^{36} + 7x^{35} - x^{34} + 4x^{33} + 3x^{32} + x^{31} + 2x^{30} - 4x^{29} - x^{28} - 2x^{27}) q^{68} \\
& + (-x^{37} + 5x^{35} - 2x^{34} + 11x^{33} - x^{32} - 4x^{31} + 3x^{30} - 3x^{29} + 2x^{28} + x^{27}) q^{67} \\
& + (-3x^{37} + 4x^{35} - x^{34} + 9x^{33} + 2x^{31} + x^{30} - 5x^{29} + x^{28} - x^{27} + x^{26}) q^{66} \\
& + (-x^{37} + 3x^{35} - 2x^{34} + 7x^{33} - 3x^{32} - 3x^{31} + 2x^{30} - 3x^{29} + 3x^{28} + x^{27} - 2x^{26}) q^{65} \\
& + (-2x^{37} - 3x^{34} + 4x^{33} - 2x^{32} - x^{31} + x^{30} - 8x^{29} + x^{28} + x^{26} + 2x^{25}) q^{64} \\
& + (x^{37} + x^{35} - x^{34} + 5x^{33} + x^{32} - 7x^{31} + 3x^{30} - 6x^{29} - x^{27} - x^{26} - x^{25}) q^{63} \\
& + (-x^{37} + 3x^{35} + 6x^{33} - 6x^{31} + 3x^{30} - 11x^{29} + 3x^{28} - x^{27} + x^{26} + 2x^{25} - 2x^{24}) q^{62} \\
& + (-x^{35} + 5x^{33} - 2x^{31} + 7x^{30} - 9x^{29} + 3x^{28} - 2x^{27} - 3x^{26} + x^{24}) q^{61} \\
& + (x^{35} + 5x^{33} + 7x^{30} - 11x^{29} + 4x^{28} - x^{26} + 3x^{25} - 2x^{24} - x^{23}) q^{60} \\
& + (-x^{35} + 3x^{33} + 2x^{30} - 6x^{29} + 3x^{28} - 2x^{27} + 3x^{25} + 2x^{23} - x^{22}) q^{59} \\
& + (2x^{35} + 3x^{33} - 2x^{32} - 2x^{31} + 3x^{30} - 6x^{29} + 2x^{28} - 3x^{26} + 3x^{25} - 3x^{24} - x^{23} + 2x^{22}) q^{58} \\
& + (-x^{35} + 3x^{33} - x^{32} + x^{30} - 11x^{29} + x^{28} - 4x^{26} + 5x^{25} - 3x^{24} + x^{23} - x^{22}) q^{57} \\
& + (-x^{32} - 2x^{31} + 3x^{30} - 9x^{29} - x^{28} - 2x^{27} - 5x^{26} + 5x^{25} - 3x^{24} - x^{23} + x^{22}) q^{56} \\
& + (2x^{33} - x^{31} + x^{30} - 11x^{29} + 4x^{28} - 6x^{27} - 7x^{26} + 6x^{25} - 5x^{24} + 3x^{23} - x^{22} - x^{21} + x^{20}) q^{55} \\
& + (-x^{33} - x^{31} + 4x^{30} - 6x^{29} + 3x^{28} - 7x^{27} - 4x^{26} + 5x^{25} - 5x^{24} + x^{23} + x^{21}) q^{54} \\
& + (2x^{33} + x^{30} - 8x^{29} + 6x^{28} - x^{27} - 3x^{26} + 4x^{25} - 6x^{24} + x^{22} - 2x^{21} + 2x^{20}) q^{53} \\
& + (x^{31} + 2x^{30} - 3x^{29} + x^{28} - 3x^{27} - x^{26} + 7x^{25} - 5x^{24} + 3x^{23} + x^{22} - x^{21}) q^{52} \\
& + (-x^{31} - 5x^{29} + 4x^{28} + 2x^{27} - 8x^{26} + 9x^{25} - 4x^{24} + 4x^{23} + 2x^{22} - 3x^{21} + 2x^{20}) q^{51} \\
& + (x^{31} - 3x^{29} - x^{28} - 4x^{27} - 4x^{26} + 11x^{25} - 7x^{24} + 5x^{23} - x^{21} + 4x^{20} + x^{18}) q^{50} \\
& + (-2x^{31} - 4x^{29} + 3x^{28} + x^{27} - 9x^{26} + 4x^{25} - 9x^{24} + 7x^{23} + 2x^{22} + 3x^{20} + x^{19} - x^{18}) q^{49} \\
& + (x^{31} - 2x^{29} + x^{28} - 5x^{27} - 2x^{26} + 7x^{25} - 11x^{24} + 4x^{23} - 3x^{21} + 5x^{20} - x^{19}) q^{48} \\
& + (2x^{28} - 5x^{26} + 2x^{25} - 4x^{24} + 3x^{23} - 3x^{21} + 3x^{20} + x^{18}) q^{47} \\
& + (-2x^{29} + x^{28} - x^{27} + x^{26} + 8x^{25} - 7x^{24} + x^{23} + 2x^{22} - 4x^{21} + 8x^{20} - 2x^{19} - x^{18} - x^{16}) q^{46} \\
& + (x^{28} + x^{27} - 3x^{26} + 3x^{25} - 2x^{24} + 8x^{23} + 6x^{22} - 3x^{21} + 6x^{20} - 3x^{19} + x^{18} - x^{16}) q^{45} \\
& + (-x^{29} - x^{27} + 8x^{25} - 8x^{24} + 4x^{23} + 7x^{22} - 2x^{21} + 11x^{20} - x^{19} + x^{17} - x^{16}) q^{44} \\
& + (-2x^{26} + 2x^{25} - 3x^{24} + 9x^{23} + x^{22} - x^{21} + 9x^{20} - 2x^{19} + 5x^{18} - 2x^{16}) q^{43} \\
& + (x^{27} + 4x^{25} - 8x^{24} + 2x^{23} + 3x^{22} + x^{21} + 11x^{20} - x^{19} - x^{18} + x^{17} - x^{16}) q^{42} \\
& + (-x^{27} - x^{26} + x^{25} - 2x^{24} + 5x^{23} - 2x^{22} - 4x^{21} + 6x^{20} - 3x^{19} + 4x^{18} + 2x^{17} - 4x^{16}) q^{41} \\
& + (2x^{25} - 4x^{24} - x^{23} + 4x^{22} - 3x^{21} + 6x^{20} - 3x^{19} - 2x^{18} - 2x^{16} - x^{14}) q^{40}
\end{aligned}$$

$$\begin{aligned}
& + (x^{25} - x^{24} + 3x^{23} - x^{22} - 6x^{21} + 11x^{20} - 7x^{19} + 3x^{18} + x^{17} - 8x^{16}) q^{39} \\
& + (x^{25} - 2x^{24} + 5x^{22} - x^{21} + 9x^{20} - 7x^{19} + x^{18} - 3x^{17} - 3x^{16} - 2x^{14}) q^{38} \\
& + (x^{25} - x^{24} + 2x^{23} - 4x^{21} + 11x^{20} - 2x^{19} + 7x^{18} + x^{17} - 8x^{16} - x^{15}) q^{37} \\
& + (-x^{24} + x^{22} + x^{21} + 6x^{20} - 3x^{19} + 6x^{18} - 2x^{16} + 2x^{15} - 3x^{14} + x^{12}) q^{36} \\
& + (-x^{24} + x^{23} - x^{22} - 3x^{21} + 8x^{20} - x^{19} + 2x^{18} + 3x^{17} - 7x^{16} + 2x^{15} + x^{14} + x^{12}) q^{35} \\
& + (x^{22} - x^{21} + 3x^{20} - 3x^{19} + 2x^{17} - 4x^{16} + 4x^{15} - 5x^{14} + 2x^{12}) q^{34} \\
& + (-2x^{21} + 5x^{20} - x^{19} - x^{17} - 11x^{16} - 2x^{14} + x^{12}) q^{33} \\
& + (-x^{22} - x^{21} + 3x^{20} - 4x^{19} + 2x^{18} - 9x^{16} + 2x^{15} - 9x^{14} - x^{13} + 3x^{12}) q^{32} \\
& + (x^{22} - x^{21} + 4x^{20} - x^{19} - 7x^{16} - x^{15} - 4x^{14} - x^{13} - x^{12}) q^{31} \\
& + (2x^{20} - 2x^{19} + 2x^{18} - 4x^{16} + x^{15} - 8x^{14} - x^{13} + 4x^{12}) q^{30} \\
& + (x^{18} - 5x^{16} + 2x^{15} - x^{14} + 2x^{13} + x^{12} + 2x^{10}) q^{29} \\
& + (2x^{20} + x^{18} + 2x^{17} - 6x^{16} + x^{15} - 3x^{14} - x^{13} + 6x^{12} + x^{10}) q^{28} \\
& + (x^{17} - 5x^{16} + 2x^{15} - 4x^{14} + x^{13} + 3x^{12} + 4x^{10}) q^{27} \\
& + (x^{20} - x^{18} + x^{17} - 5x^{16} + 3x^{15} - 7x^{14} + 4x^{12} + x^{10}) q^{26} \\
& + (x^{18} - 3x^{16} + x^{15} - 5x^{14} + x^{13} - x^{12} - x^{11} + 3x^{10} - x^8) q^{25} \\
& + (-x^{18} - 3x^{16} - 4x^{14} + x^{12} + x^{11} + x^{10} - x^8) q^{24} \\
& + (2x^{18} - 3x^{16} - 3x^{14} - x^{13} + 2x^{12} - 2x^{11} + 3x^{10} - 2x^8) q^{23} \\
& + (-x^{18} - x^{13} + 3x^{12} - x^{11} + 2x^{10}) q^{22} + (-2x^{16} - x^{14} + 4x^{12} - x^{11} + 7x^{10}) q^{21} \\
& + (x^{16} - 3x^{14} + 3x^{12} + 7x^{10}) q^{20} + (-2x^{16} + x^{14} + 3x^{12} + 3x^{10} + x^9) q^{19} \\
& + (-x^{14} + 3x^{10} + x^8 - x^6) q^{18} + (x^{14} + x^{12} + x^{10} - 2x^8 - 3x^6) q^{17} \\
& + (-2x^{14} + 3x^{12} + 2x^{10} - 3x^8 - 2x^6) q^{16} + (x^{14} + x^{12} + x^{10} - x^6) q^{15} \\
& + (2x^{12} + 3x^{10} - x^8 - 2x^6) q^{14} + (-x^{12} + 2x^{10} + 3x^8 - x^6 + x^4) q^{13} \\
& + (x^{12} - x^8 + x^6 + x^4) q^{12} + (x^{10} - 2x^6) q^{11} + (-x^{10} - 2x^8 - x^4) q^{10} \\
& + (-x^8 - 4x^6) q^9 + (-2x^6 - x^4) q^8 + (-x^8 - 2x^6 + x^4) q^7 + (x^6 - 2x^4 + x^2) q^6 \\
& + (x^4 + x^2) q^5 + (x^4 + 2x^2) q^4 + (x^4 - x^2) q^3 + x^2 q^2 - 1.
\end{aligned}$$

$$\delta(x, q) = \frac{N(\delta)}{D(\delta)},$$

$$\begin{aligned}
D(\delta) = & q^{129/2} x^{31} - 2q^{125/2} x^{29} - 2q^{67/2} x^{11} + q^{63/2} x^9 + q^{123/2} x^9 (x^{20} - x^{18}) \\
& + q^{121/2} x^9 (x^{18} - 2x^{20}) + q^{119/2} x^9 (x^{16} - 2x^{18}) \\
& + q^{117/2} x^9 (4x^{18} - 2x^{16}) + q^{115/2} x^9 (4x^{16} - 2x^{18}) \\
& + q^{77/2} x^9 (4x^6 - 2x^4) + q^{75/2} x^9 (4x^4 - 2x^6) + q^{73/2} x^9 (x^6 - 2x^4) \\
& + q^{71/2} x^9 (x^4 - 2x^2) + q^{69/2} x^9 (x^2 - x^4) + q^{113/2} x^9 (x^{18} - 3x^{16} + 2x^{14}) \\
& + q^{111/2} x^9 (-x^{18} + 4x^{16} - 3x^{14}) + q^{109/2} x^9 (-3x^{16} + 5x^{14} - x^{12})
\end{aligned}$$

$$\begin{aligned}
& + q^{107/2} x^9 (4x^{16} - 5x^{14} + 2x^{12}) + q^{105/2} x^9 (-2x^{16} + 5x^{14} - 4x^{12}) \\
& + q^{101/2} x^9 (5x^{14} - 7x^{12} + 2x^{10}) + q^{99/2} x^9 (-3x^{14} + 7x^{12} - 4x^{10}) \\
& + q^{97/2} x^9 (2x^{14} - 7x^{12} + 4x^{10}) + q^{95/2} x^9 (4x^{12} - 7x^{10} + 2x^8) \\
& + q^{93/2} x^9 (-4x^{12} + 7x^{10} - 3x^8) + q^{91/2} x^9 (2x^{12} - 7x^{10} + 5x^8) \\
& + q^{87/2} x^9 (-4x^{10} + 5x^8 - 2x^6) + q^{85/2} x^9 (2x^{10} - 5x^8 + 4x^6) \\
& + q^{83/2} x^9 (-x^{10} + 5x^8 - 3x^6) + q^{81/2} x^9 (-3x^8 + 4x^6 - x^4) \\
& + q^{79/2} x^9 (2x^8 - 3x^6 + x^4) + q^{103/2} x^9 (x^{16} - 5x^{14} + 4x^{12} - x^{10}) \\
& + q^{89/2} x^9 (-x^{12} + 4x^{10} - 5x^8 + x^6)
\end{aligned}$$

$$\begin{aligned}
N(\delta) = & -x^{39} q^{83} + 2x^{37} q^{81} + (x^{35} - x^{37}) q^{80} + (2x^{37} - x^{35}) q^{79} + (x^{37} + 2x^{35} - x^{33}) q^{78} \\
& + (x^{37} - 4x^{35} + 2x^{33}) q^{77} - 4x^{33} q^{76} + (-2x^{35} + 2x^{33} - 2x^{31}) q^{75} \\
& + (3x^{31} - 4x^{33}) q^{74} + (-x^{35} + 2x^{33} - 4x^{31} + x^{29}) q^{73} + (-2x^{33} + 4x^{31} - 2x^{29}) q^{72} \\
& + (x^{35} + 2x^{33} - 3x^{31} + 4x^{29}) q^{71} + (x^{35} - x^{33} + 5x^{31} - 2x^{29} + x^{27}) q^{70} \\
& + (-3x^{33} - 3x^{31} + 6x^{29} - 2x^{27}) q^{69} + (-2x^{33} + x^{31} - 4x^{29} + 3x^{27}) q^{68} \\
& + (-2x^{33} + 5x^{29} - 3x^{27}) q^{67} + (-3x^{33} + 5x^{27} - 2x^{25}) q^{66} \\
& + (-x^{33} + 3x^{31} + 3x^{29} - 5x^{27} + 2x^{25}) q^{65} \\
& + (3x^{31} + 3x^{29} + 3x^{27} - 4x^{25}) q^{64} + (x^{31} + 4x^{29} + 2x^{25} - x^{23}) q^{63} \\
& + (4x^{29} + x^{27} - 4x^{25} + 2x^{23}) q^{62} + (x^{29} - x^{27} - 2x^{23}) q^{61} \\
& + (-2x^{31} + 3x^{29} - 2x^{27} - 4x^{25} + x^{23}) q^{60} \\
& + (-x^{31} + x^{29} - 3x^{25} - 3x^{23} + x^{21}) q^{59} + (-x^{31} + 5x^{29} - 4x^{27} - 3x^{25} + x^{23}) q^{58} \\
& + (2x^{29} + 3x^{27} - 7x^{25} - 2x^{23} + 2x^{21}) q^{57} + (5x^{29} - 2x^{27} - 2x^{23} - x^{21}) q^{56} \\
& + (x^{29} + 4x^{27} - 6x^{25} + x^{23} + 3x^{21}) q^{55} + (2x^{29} - 4x^{27} + x^{25} - 5x^{23} + 3x^{21} + x^{19}) q^{54} \\
& + (3x^{27} - 12x^{25} + 2x^{23} + x^{21} - x^{19}) q^{53} + (-3x^{27} - 8x^{23} + 5x^{21} + x^{19}) q^{52} \\
& + (3x^{27} - 12x^{25} + 3x^{23} + 2x^{19}) q^{51} + (x^{27} + x^{25} - 11x^{23} + 8x^{21} - x^{17}) q^{50} \\
& + (2x^{27} - 8x^{25} + 8x^{23} - 3x^{21} + 3x^{19} - x^{17}) q^{49} + (x^{27} - 8x^{23} + 13x^{21} - x^{17}) q^{48} \\
& + (x^{27} - 5x^{25} + 6x^{23} - 2x^{21} + 9x^{19} - 2x^{17}) q^{47} \\
& + (-x^{25} - 8x^{23} + 15x^{21} - 2x^{19}) q^{46} + (-3x^{25} + 2x^{23} - 5x^{21} + 11x^{19} - 4x^{17}) q^{45} \\
& + (-7x^{23} + 11x^{21} - 4x^{19} + x^{17} - x^{15}) q^{44} + (-x^{25} + x^{23} - 4x^{21} + 11x^{19} - 7x^{17}) q^{43} \\
& + (-4x^{23} + 11x^{21} - 5x^{19} + 2x^{17} - 3x^{15}) q^{42} + (-2x^{21} + 15x^{19} - 8x^{17} - x^{15}) q^{41} \\
& + (-2x^{23} + 9x^{21} - 2x^{19} + 6x^{17} - 5x^{15} + x^{13}) q^{40} + (-x^{23} + 13x^{19} - 8x^{17} + x^{13}) q^{39} \\
& + (-x^{23} + 3x^{21} - 3x^{19} + 8x^{17} - 8x^{15} + 2x^{13}) q^{38} + (-x^{23} + 8x^{19} - 11x^{17} + x^{15} + x^{13}) q^{37} \\
& + (2x^{21} + 3x^{17} - 12x^{15} + 3x^{13}) q^{36} + (x^{21} + 5x^{19} - 8x^{17} - 3x^{13}) q^{35} \\
& + (-x^{21} + x^{19} + 2x^{17} - 12x^{15} + 3x^{13}) q^{34} \\
& + (x^{22} + x^{21} + 3x^{19} - 5x^{17} + x^{15} - 4x^{13} + 2x^{11}) q^{33} \\
& + (3x^{19} + x^{17} - 6x^{15} + 4x^{13} + x^{11}) q^{32} + (-2x^{20} - x^{19} - 2x^{17} - 2x^{13} + 5x^{11}) q^{31}
\end{aligned}$$

$$\begin{aligned}
& + (x^{20} + 2x^{19} - x^{18} - 2x^{17} - 7x^{15} + 3x^{13} + 2x^{11}) q^{30} \\
& + (-2x^{20} + x^{18} + x^{17} - 3x^{15} - 4x^{13} + 5x^{11} - x^9) q^{29} \\
& + (x^{19} - 2x^{18} - 3x^{17} + x^{16} - 3x^{15} + x^{11} - x^9) q^{28} \\
& + (4x^{18} + x^{17} - 2x^{16} - 4x^{15} - 2x^{13} + 3x^{11} - 2x^9) q^{27} \\
& + (-2x^{18} - 2x^{17} + 4x^{16} - x^{13} + x^{11}) q^{26} \\
& + (x^{18} + 2x^{17} - 3x^{16} - 4x^{15} + 2x^{14} + x^{13} + 4x^{11}) q^{25} \\
& + (-x^{18} - x^{17} + 4x^{16} + 2x^{15} - 3x^{14} + 4x^{11} + x^9) q^{24} \\
& + (-3x^{16} - 4x^{15} + 5x^{14} + 3x^{13} - x^{12} + 3x^{11} + 3x^9) q^{23} \\
& + (4x^{16} + 2x^{15} - 5x^{14} - 5x^{13} + 2x^{12} + 3x^{11} + 3x^9 - x^7) q^{22} \\
& + (-2x^{16} - 2x^{15} + 5x^{14} + 5x^{13} - 4x^{12} - 3x^7) q^{21} \\
& + (x^{16} - 5x^{14} - 3x^{13} + 4x^{12} + 5x^{11} - x^{10} - 2x^7) q^{20} \\
& + (5x^{14} + 3x^{13} - 7x^{12} - 4x^{11} + 2x^{10} + x^9 - 2x^7) q^{19} \\
& + (-3x^{14} - 2x^{13} + 7x^{12} + 6x^{11} - 4x^{10} - 3x^9 - 3x^7) q^{18} \\
& + (2x^{14} + x^{13} - 7x^{12} - 2x^{11} + 4x^{10} + 5x^9 - x^7 + x^5) q^{17} \\
& + (4x^{12} + 4x^{11} - 7x^{10} - 3x^9 + 2x^8 + 2x^7 + x^5) q^{16} \\
& + (-4x^{12} - 2x^{11} + 7x^{10} + 4x^9 - 3x^8 - 2x^7) q^{15} \\
& + (2x^{12} + x^{11} - 7x^{10} - 4x^9 + 5x^8 + 2x^7 - x^5) q^{14} \\
& + (-x^{12} + 4x^{10} + 3x^9 - 5x^8 - 4x^7 + x^6) q^{13} + (-4x^{10} - 2x^9 + 5x^8 + 2x^7 - 2x^6 - 2x^5) q^{12} \\
& + (2x^{10} - 5x^8 - 4x^7 + 4x^6) q^{11} + (-x^{10} + 5x^8 + 2x^7 - 3x^6 - 4x^5 + x^3) q^{10} \\
& + (-3x^8 - x^7 + 4x^6 + 2x^5 - x^4 + x^3) q^9 + (2x^8 - 3x^6 - x^5 + x^4 + 2x^3) q^8 \\
& + (4x^6 + x^5 - 2x^4 - x^3) q^7 + (-2x^6 + 4x^4 + 2x^3) q^6 + (x^6 - 2x^4) q^5 \\
& + (x^4 - 2x^2 - x) q^4 + (x^2 - x^4) q^3 - 2x^2 q^2 + 1.
\end{aligned}$$

The  $\hbar$  expansions of the above coefficients functions are the following.

$$\begin{aligned}
\alpha(x, e^{\hbar}) = & -\frac{1}{x^9} + \frac{(5x^{16} - 2x^{14} - 37x^{12} - 40x^{10} + 28x^8 + 104x^6 + 71x^4 - 2x^2 - 31)}{x^9(x^2 - 1)(x^2 + 1)(x^{12} - 2x^8 - 4x^6 - 2x^4 + 1)} \hbar \\
& + \frac{1}{2x^9(x^2 - 1)(x^2 + 1)^2(x^{12} - 2x^8 - 4x^6 - 2x^4 + 1)^2} \left( -25x^{30} + 11x^{28} + 729x^{26} \right. \\
& + 1509x^{24} - 1068x^{22} - 8092x^{20} - 9514x^{18} + 5430x^{16} + 27546x^{14} + 31834x^{12} + 12988x^{10} \\
& \left. - 7284x^8 - 10941x^6 - 3681x^4 + 1069x^2 + 961 \right) \hbar^2 + O(\hbar^3)
\end{aligned}$$

$$\begin{aligned}
\beta(x, e^{\hbar}) = & \frac{1}{x^{17}} (-x^{17} + x^{16} - 2x^{14} - 3x^{12} + 2x^{10} + 7x^8 + 2x^6 - 3x^4 - 2x^2 + 1) \\
& - \frac{1}{2x^{17}(x^{16} - 3x^{12} - 4x^{10} + 4x^6 + 3x^4 - 1)} \left( -x^{33} + x^{32} + 4x^{31} - 16x^{30} + 47x^{29} \right. \\
& \left. - 68x^{28} + 44x^{27} + 116x^{26} - 56x^{25} + 538x^{24} - 172x^{23} + 156x^{22} - 115x^{21} - 1439x^{20} \right.
\end{aligned}$$



$$\begin{aligned}
& + 4x^{19} - 1936x^{18} + 53x^{17} + 460x^{16} + 2924x^{14} + 1891x^{12} - 924x^{10} - 1622x^8 - 244x^6 \\
& + 472x^4 + 164x^2 - 89) \hbar \\
& + \frac{1}{8x^{17}(x^{16} - 3x^{12} - 4x^{10} + 4x^6 + 3x^4 - 1)^2} \left( -x^{49} + x^{48} + 72x^{47} - 146x^{46} + 1486x^{45} \right. \\
& - 1561x^{44} + 1824x^{43} + 3126x^{42} - 5745x^{41} + 21810x^{40} - 16576x^{39} + 2724x^{38} - 1926x^{37} \\
& - 123674x^{36} + 40840x^{35} - 171040x^{34} + 58980x^{33} + 217052x^{32} + 8872x^{31} + 754786x^{30} \\
& - 54198x^{29} + 388419x^{28} - 56320x^{27} - 1005850x^{26} - 8985x^{25} - 1674366x^{24} + 21264x^{23} \\
& - 305650x^{22} + 13582x^{21} + 1557339x^{20} - 360x^{19} + 1533466x^{18} - 2809x^{17} - 91108x^{16} \\
& - 1042960x^{14} - 532634x^{12} + 214404x^{10} + 281730x^8 + 22926x^6 - 61681x^4 - 13466x^2 \\
& \left. + 7921 \right) \hbar^2 + O(\hbar^3)
\end{aligned}$$

$$\begin{aligned}
\gamma(x, e^{\hbar}) &= -\frac{1}{x^{17}} + \frac{2}{x^{15}} + \frac{3}{x^{13}} - \frac{2}{x^{11}} - \frac{7}{x^9} + x^8 + \frac{1}{x^8} - \frac{2}{x^7} - 2x^6 - \frac{2}{x^6} + \frac{3}{x^5} - 3x^4 - \frac{3}{x^4} + \frac{2}{x^3} \\
& + 2x^2 + \frac{2}{x^2} - \frac{1}{x} + 7 \\
& + \frac{1}{x^{17}(x^{16} - 3x^{12} - 4x^{10} + 4x^6 + 3x^4 - 1)} \left( 13x^{41} - 19x^{39} - 47x^{37} - 4x^{35} + 55x^{33} + 4x^{32} \right. \\
& + 84x^{31} - 19x^{30} + 220x^{29} - 59x^{28} + 239x^{27} + 86x^{26} - 230x^{25} + 401x^{24} - 733x^{23} \\
& + 134x^{22} - 446x^{21} - 913x^{20} + 300x^{19} - 1251x^{18} + 487x^{17} + 198x^{16} + 68x^{15} + 1665x^{14} \\
& \left. - 155x^{13} + 1085x^{12} - 55x^{11} - 514x^{10} + 31x^9 - 895x^8 - 130x^6 + 265x^4 + 89x^2 - 50 \right) \hbar \\
& - \frac{1}{2x^{17}(x+1)^2(x^2+1)^2(x^2+x+1)^2(x^{10}-x^9+x^7-3x^6+2x^5-3x^4+x^3-x+1)^2} \\
& \times \left( -169x^{55} - 338x^{54} - 322x^{53} - 306x^{52} + 782x^{51} + 1870x^{50} + 3243x^{49} + 4616x^{48} \right. \\
& + 2305x^{47} + 10x^{46} - 6935x^{45} - 14061x^{44} - 14879x^{43} - 16534x^{42} - 1889x^{41} + 14715x^{40} \\
& + 25683x^{39} + 47565x^{38} + 23918x^{37} + 1153x^{36} - 45216x^{35} - 145535x^{34} - 170229x^{33} \\
& - 268495x^{32} - 246695x^{31} - 146963x^{30} - 41626x^{29} + 348444x^{28} + 598018x^{27} \\
& + 1011439x^{26} + 1301463x^{25} + 1268658x^{24} + 1261033x^{23} + 686816x^{22} + 216091x^{21} \\
& - 382307x^{20} - 933501x^{19} - 1003328x^{18} - 1098973x^{17} - 710409x^{16} - 351521x^{15} \\
& - 16653x^{14} + 316520x^{13} + 329665x^{12} + 349894x^{11} + 209685x^{10} + 70993x^9 + 1007x^8 \\
& - 69940x^7 - 54805x^6 - 39670x^5 - 18796x^4 + 2078x^3 + 3539x^2 + 5000x + 2500 \left. \right) \hbar^2 \\
& + O(\hbar^3)
\end{aligned}$$

$$\begin{aligned}
\delta(x, e^{\hbar}) &= \frac{1}{x^9} - x^8 - \frac{1}{x^8} + 2x^6 + \frac{2}{x^6} + 3x^4 + \frac{3}{x^4} - 2x^2 - \frac{2}{x^2} - 7 \\
& - \frac{1}{2x^9(x^{16} - 3x^{12} - 4x^{10} + 4x^6 + 3x^4 - 1)} \left( 37x^{33} - 52x^{31} - 152x^{29} + 8x^{27} + 278x^{25} \right.
\end{aligned}$$

$$\begin{aligned}
& + 272x^{23} + 161x^{21} + 72x^{19} - 396x^{17} + 63x^{16} - 900x^{15} - 505x^{13} - 189x^{12} + 488x^{11} \\
& - 252x^{10} + 710x^9 + 80x^7 + 252x^6 - 260x^5 + 189x^4 - 88x^3 + 55x - 63 \Big) \hbar \\
& + \frac{1}{8x^9(x^{16} - 3x^{12} - 4x^{10} + 4x^6 + 3x^4 - 1)^2} \Big( -1369x^{49} + 1354x^{47} + 8793x^{45} + 2874x^{43} \\
& - 27186x^{41} - 37188x^{39} + 24730x^{37} + 92688x^{35} + 28292x^{33} + 3969x^{32} - 127602x^{31} \\
& - 110123x^{29} - 23814x^{28} + 143906x^{27} - 31752x^{26} + 276198x^{25} + 35721x^{24} + 13802x^{23} \\
& + 127008x^{22} - 321803x^{21} + 87318x^{20} - 260586x^{19} - 95256x^{18} + 96260x^{17} \\
& - 206388x^{16} + 256992x^{15} - 95256x^{14} + 95722x^{13} + 87318x^{12} - 82404x^{11} + 127008x^{10} \\
& - 77298x^9 + 35721x^8 + 354x^7 - 31752x^6 + 21177x^5 - 23814x^4 + 3874x^3 - 3025x \\
& + 3969 \Big) \hbar^2 + O(\hbar^3).
\end{aligned}$$

## References

- [1] Chae J., A Cable Knot and BPS Series, arXiv (January 2021)
