# Supplementary material for: A Cable Knot and BPS-Series
Source: arXiv:2101.11708 ancillary file (2023-01-18)
Supplement: Supplementary file 2 [file Recursion_Relation_2.pdf]

## The Definitions of the Coefficients in the Recursion Relation

John Chae

Department of Physics and QMAP, UC Davis, 1 Shields Ave, Davis, CA, 95616, USA  
yjchae@ucdavis.edu

This is a list of the coefficient functions  $t_v(q, q^m)$  of the  $f_m$ -recursion relation (9) in Section 4 in [1].

$$\begin{aligned}
 t_2(q, q^m) &= q^{\frac{m+109}{2}} \left( q^{\frac{m+83}{2}} - q^{\frac{m+85}{2}} + 2q^{\frac{m+87}{2}} + q^{\frac{m+89}{2}} + q^{\frac{m+91}{2}} - q^4 + q^3 - 2q^2 - q - 1 \right) \\
 t_4(q, q^m) &= q^{\frac{m+107}{2}} \left( q^{\frac{m+79}{2}} + q^{\frac{m+81}{2}} + q^{\frac{m+83}{2}} - 2q^{\frac{m+85}{2}} + q^{\frac{m+87}{2}} - q^{\frac{m+89}{2}} - q^{\frac{m+93}{2}} + q^{\frac{m+97}{2}} + q^{\frac{m+99}{2}} \right. \\
 &\quad \left. - q^{10} - q^9 - q^8 + 2q^7 - q^6 + q^5 + q^3 - q - 1 \right) \\
 t_6(q, q^m) &= -q^{\frac{m+109}{2}} \left( -q^{\frac{m+75}{2}} + 2q^{\frac{m+77}{2}} + 2q^{\frac{m+79}{2}} + 4q^{\frac{m+81}{2}} + 2q^{\frac{m+85}{2}} - q^{\frac{m+87}{2}} + q^{\frac{m+89}{2}} + 2q^{\frac{m+91}{2}} \right. \\
 &\quad \left. + q^{\frac{m+93}{2}} + 2q^{\frac{m+95}{2}} + 3q^{\frac{m+97}{2}} + q^{\frac{m+99}{2}} + q^{12} - 2q^{11} - 2q^{10} - 4q^9 - 2q^7 + q^6 - q^5 - 2q^4 \right. \\
 &\quad \left. - q^3 - 2q^2 - 3q - 1 \right) \\
 t_8(q, q^m) &= -q^{m+89} - q^{m+91} - 2q^{m+92} - q^{m+94} + 3q^{m+95} - q^{m+96} - 3q^{m+98} - 2q^{m+99} + q^{m+100} \\
 &\quad - 2q^{m+105} - q^{m+106} - q^{m+107} + q^{\frac{3m}{2} + \frac{283}{2}} + q^{\frac{m+107}{2}} + q^{\frac{m+109}{2}} + 2q^{\frac{m+111}{2}} - q^{\frac{m+121}{2}} \\
 &\quad + 2q^{\frac{m+123}{2}} + 3q^{\frac{m+125}{2}} + q^{\frac{m+129}{2}} - 3q^{\frac{m+131}{2}} + q^{\frac{m+133}{2}} + 2q^{\frac{m+137}{2}} + q^{\frac{m+139}{2}} + q^{\frac{m+143}{2}} - q^{19} \\
 t_9(q, q^m) &= q^{m+99} - q^{\frac{3(m+95)}{2}} \\
 t_{10}(q, q^m) &= -q^{23} \left( q^{m+65} - q^{m+66} - 2q^{m+68} - 3q^{m+69} - q^{m+70} - 2q^{m+71} - q^{m+72} - 3q^{m+73} \right. \\
 &\quad - 3q^{m+74} - 7q^{m+75} - 7q^{m+76} - 2q^{m+77} - 3q^{m+78} - q^{m+79} - 3q^{m+80} - q^{m+81} - 4q^{m+82} \\
 &\quad - q^{m+83} - 2q^{m+84} + q^{\frac{3m}{2} + \frac{229}{2}} + 2q^{\frac{3m}{2} + \frac{233}{2}} + 2q^{\frac{m+65}{2}} + q^{\frac{m+67}{2}} + 4q^{\frac{m+69}{2}} + q^{\frac{m+71}{2}} \\
 &\quad + 3q^{\frac{m+73}{2}} + q^{\frac{m+75}{2}} + 3q^{\frac{m+77}{2}} - q^{\frac{3(m+77)}{2}} + 2q^{\frac{m+79}{2}} + 7q^{\frac{m+81}{2}} + 7q^{\frac{m+83}{2}} + 3q^{\frac{m+85}{2}} + 3q^{\frac{m+87}{2}} \\
 &\quad \left. + q^{\frac{m+89}{2}} + 2q^{\frac{m+91}{2}} + q^{\frac{m+93}{2}} + 3q^{\frac{m+95}{2}} + 2q^{\frac{m+97}{2}} + q^{\frac{m+101}{2}} - q^{\frac{m+103}{2}} - q^2 + q - 2 \right) \\
 t_{11}(q, q^m) &= q^{m+89} \left( q^{\frac{m+99}{2}} - q^{\frac{m+101}{2}} + 2q^{\frac{m+103}{2}} + q^{\frac{m+105}{2}} + q^{\frac{m+107}{2}} - q^{12} + q^{11} - 2q^{10} - q^9 - q^8 \right) \\
 t_{12}(q, q^m) &= -q^{26} \left( -q^{m+60} + q^{m+61} - 2q^{m+62} - q^{m+63} - 3q^{m+64} - q^{m+65} - 3q^{m+67} - 3q^{m+68} \right. \\
 &\quad - 4q^{m+69} - 3q^{m+70} - 2q^{m+71} - q^{m+72} + q^{m+73} - 4q^{m+74} - 3q^{m+75} - 6q^{m+76} - q^{m+77} \\
 &\quad - 4q^{m+78} + q^{m+79} - 3q^{m+80} - q^{m+81} - 2q^{m+82} - q^{m+83} - q^{m+84} + q^{\frac{3m}{2} + \frac{215}{2}} \\
 &\quad + q^{\frac{3m}{2} + \frac{217}{2}} + 2q^{\frac{3m}{2} + \frac{221}{2}} - q^{\frac{3m}{2} + \frac{223}{2}} + q^{\frac{m+57}{2}} + q^{\frac{m+59}{2}} + 2q^{\frac{m+61}{2}} + q^{\frac{m+63}{2}} + 3q^{\frac{m+65}{2}} \\
 &\quad - q^{\frac{m+67}{2}} + 4q^{\frac{m+69}{2}} + q^{\frac{m+71}{2}} + q^{\frac{3(m+71)}{2}} + 6q^{\frac{m+73}{2}} - 2q^{\frac{3(m+73)}{2}} + 3q^{\frac{m+75}{2}} + q^{\frac{3(m+75)}{2}} \\
 &\quad + 4q^{\frac{m+77}{2}} - q^{\frac{m+79}{2}} + q^{\frac{m+81}{2}} + 2q^{\frac{m+83}{2}} + 3q^{\frac{m+85}{2}} + 4q^{\frac{m+87}{2}} + 3q^{\frac{m+89}{2}} + 3q^{\frac{m+91}{2}} + q^{\frac{m+95}{2}} \\
 &\quad \left. + 3q^{\frac{m+97}{2}} + q^{\frac{m+99}{2}} + 2q^{\frac{m+101}{2}} - q^{\frac{m+103}{2}} + q^{\frac{m+105}{2}} - q^6 - q^5 - q^4 + 2q^3 - 2q^2 + q - 1 \right)
 \end{aligned}$$

$$\begin{aligned}
t_{13}(q, q^m) &= q^{m+84} \left( q^{\frac{m+99}{2}} + q^{\frac{m+101}{2}} + q^{\frac{m+103}{2}} - 2q^{\frac{m+105}{2}} + q^{\frac{m+107}{2}} - q^{\frac{m+109}{2}} - q^{\frac{m+113}{2}} + q^{\frac{m+117}{2}} \right. \\
&\quad \left. + q^{\frac{m+119}{2}} - q^{20} - q^{19} - q^{18} + 2q^{17} - q^{16} + q^{15} + q^{13} - q^{11} - q^{10} \right) \\
t_{14}(q, q^m) &= q^{30} \left( q^{m+55} - 2q^{m+56} + q^{m+57} - q^{m+58} + q^{m+59} - 3q^{m+60} - q^{m+61} - 3q^{m+63} - 4q^{m+64} \right. \\
&\quad - 5q^{m+65} - 7q^{m+66} - 4q^{m+67} - 3q^{m+68} - q^{m+69} - 8q^{m+70} - 4q^{m+71} - 9q^{m+72} \\
&\quad - 2q^{m+73} - 5q^{m+74} + q^{m+75} - 3q^{m+76} - 2q^{m+78} - q^{m+80} - q^{\frac{3m}{2} + \frac{199}{2}} + q^{\frac{3m}{2} + \frac{203}{2}} \\
&\quad + 2q^{\frac{3m}{2} + \frac{205}{2}} + 3q^{\frac{3m}{2} + \frac{209}{2}} - 2q^{\frac{3m}{2} + \frac{211}{2}} + q^{\frac{m+53}{2}} + 2q^{\frac{m+57}{2}} + 3q^{\frac{m+61}{2}} - q^{\frac{m+63}{2}} + 5q^{\frac{m+65}{2}} \\
&\quad + 2q^{\frac{m+67}{2}} + 2q^{\frac{3(m+67)}{2}} + 9q^{\frac{m+69}{2}} - 2q^{\frac{3(m+69)}{2}} + 4q^{\frac{m+71}{2}} + q^{\frac{3(m+71)}{2}} + 8q^{\frac{m+73}{2}} + q^{\frac{m+75}{2}} \\
&\quad + 3q^{\frac{m+77}{2}} + 4q^{\frac{m+79}{2}} + 7q^{\frac{m+81}{2}} + 5q^{\frac{m+83}{2}} + 4q^{\frac{m+85}{2}} + 3q^{\frac{m+87}{2}} + q^{\frac{m+91}{2}} + 3q^{\frac{m+93}{2}} - q^{\frac{m+95}{2}} \\
&\quad \left. + q^{\frac{m+97}{2}} - q^{\frac{m+99}{2}} + 2q^{\frac{m+101}{2}} - q^{\frac{m+103}{2}} + q^7 - 2q^6 - q^5 - 2q^4 + 2q^3 - 3q^2 + 2q - 1 \right) \\
t_{15}(q, q^m) &= q^{m+81} \left( q^{\frac{m+99}{2}} - 2q^{\frac{m+101}{2}} - 2q^{\frac{m+103}{2}} - 4q^{\frac{m+105}{2}} - 2q^{\frac{m+109}{2}} + q^{\frac{m+111}{2}} - q^{\frac{m+113}{2}} - 2q^{\frac{m+115}{2}} \right. \\
&\quad - q^{\frac{m+117}{2}} - 2q^{\frac{m+119}{2}} - 3q^{\frac{m+121}{2}} - q^{\frac{m+123}{2}} - q^{24} + 2q^{23} + 2q^{22} + 4q^{21} + 2q^{19} - q^{18} + q^{17} \\
&\quad \left. + 2q^{16} + q^{15} + 2q^{14} + 3q^{13} + q^{12} \right) \\
t_{16}(q, q^m) &= -2q^{m+85} + q^{m+86} - 2q^{m+87} - 3q^{m+89} - 3q^{m+90} - 3q^{m+91} - 5q^{m+92} - 5q^{m+93} \\
&\quad - 6q^{m+94} - 5q^{m+95} - 4q^{m+96} - 7q^{m+97} - 9q^{m+98} - 11q^{m+99} - 4q^{m+100} - 7q^{m+101} \\
&\quad - 2q^{m+102} - 8q^{m+103} - 3q^{m+104} - 8q^{m+105} - 2q^{m+106} - 4q^{m+107} - q^{m+108} - 2q^{m+109} \\
&\quad - q^{m+110} - q^{m+111} - q^{m+112} + q^{\frac{3m}{2} + \frac{253}{2}} - q^{\frac{3m}{2} + \frac{257}{2}} + 2q^{\frac{3m}{2} + \frac{259}{2}} + 3q^{\frac{3m}{2} + \frac{263}{2}} - 2q^{\frac{3m}{2} + \frac{265}{2}} \\
&\quad + q^{\frac{3(m+83)}{2}} + 2q^{\frac{3(m+85)}{2}} - q^{\frac{3(m+87)}{2}} + 2q^{\frac{3(m+89)}{2}} + q^{\frac{m+113}{2}} + q^{\frac{m+115}{2}} + q^{\frac{m+117}{2}} + 2q^{\frac{m+119}{2}} \\
&\quad + q^{\frac{m+121}{2}} + 4q^{\frac{m+123}{2}} + 2q^{\frac{m+125}{2}} + 8q^{\frac{m+127}{2}} + 3q^{\frac{m+129}{2}} + 8q^{\frac{m+131}{2}} + 2q^{\frac{m+133}{2}} + 7q^{\frac{m+135}{2}} \\
&\quad + 4q^{\frac{m+137}{2}} + 11q^{\frac{m+139}{2}} + 9q^{\frac{m+141}{2}} + 7q^{\frac{m+143}{2}} + 4q^{\frac{m+145}{2}} + 5q^{\frac{m+147}{2}} + 6q^{\frac{m+149}{2}} + 5q^{\frac{m+151}{2}} \\
&\quad + 5q^{\frac{m+153}{2}} + 3q^{\frac{m+155}{2}} + 3q^{\frac{m+157}{2}} + 3q^{\frac{m+159}{2}} + 2q^{\frac{m+163}{2}} - q^{\frac{m+165}{2}} + 2q^{\frac{m+167}{2}} - q^{44} - q^{42} \\
&\quad - 2q^{41} + q^{40} - 2q^{39} + q^{38} - 3q^{37} + 2q^{36} - 2q^{35} \\
t_{17}(q, q^m) &= q^{55} \left( q^{m+35} + q^{m+36} + 2q^{m+37} - q^{m+42} + 2q^{m+43} + 3q^{m+44} + q^{m+46} - 3q^{m+47} + q^{m+48} \right. \\
&\quad + 2q^{m+50} + q^{m+51} + q^{m+53} - q^{\frac{3m}{2} + \frac{145}{2}} - q^{\frac{3m}{2} + \frac{151}{2}} - q^{\frac{3m}{2} + \frac{155}{2}} - 2q^{\frac{3m}{2} + \frac{161}{2}} + q^{\frac{3m}{2} + \frac{163}{2}} \\
&\quad - 2q^{\frac{3m}{2} + \frac{173}{2}} - q^{\frac{3m}{2} + \frac{175}{2}} + q^{2m+123} - q^{\frac{m+1}{2}} - q^{\frac{3(m+47)}{2}} - 2q^{\frac{3(m+49)}{2}} + 3q^{\frac{3(m+51)}{2}} - 3q^{\frac{3(m+53)}{2}} \\
&\quad \left. - q^{\frac{3(m+59)}{2}} \right) \\
t_{18}(q, q^m) &= -q^{m+84} + 2q^{m+85} - q^{m+86} + q^{m+87} - q^{m+88} + q^{m+90} + q^{m+91} + 2q^{m+92} + 2q^{m+94} \\
&\quad + 2q^{m+97} + 6q^{m+98} + 7q^{m+99} + q^{m+100} + 3q^{m+101} - 2q^{m+102} + 4q^{m+103} - q^{m+104} \\
&\quad + 5q^{m+105} + q^{m+107} - q^{m+108} + q^{m+109} - q^{m+111} + q^{m+112} - q^{\frac{3m}{2} + \frac{245}{2}} + q^{\frac{3m}{2} + \frac{247}{2}} \\
&\quad - 2q^{\frac{3m}{2} + \frac{251}{2}} + 2q^{\frac{3m}{2} + \frac{253}{2}} + q^{\frac{3m}{2} + \frac{257}{2}} - 2q^{\frac{3m}{2} + \frac{259}{2}} - q^{\frac{3m}{2} + \frac{263}{2}} + q^{\frac{3(m+81)}{2}} - q^{\frac{3(m+83)}{2}} \\
&\quad - 2q^{\frac{3(m+85)}{2}} + 2q^{\frac{3(m+87)}{2}} - q^{\frac{m+117}{2}} + q^{\frac{m+119}{2}} - q^{\frac{m+123}{2}} + q^{\frac{m+125}{2}} - q^{\frac{m+127}{2}} - 5q^{\frac{m+131}{2}}
\end{aligned}$$

$$\begin{aligned}
& + q^{\frac{m+133}{2}} - 4q^{\frac{m+135}{2}} + 2q^{\frac{m+137}{2}} - 3q^{\frac{m+139}{2}} - q^{\frac{m+141}{2}} - 7q^{\frac{m+143}{2}} - 6q^{\frac{m+145}{2}} - 2q^{\frac{m+147}{2}} \\
& - 2q^{\frac{m+153}{2}} - 2q^{\frac{m+157}{2}} - q^{\frac{m+159}{2}} - q^{\frac{m+161}{2}} + q^{\frac{m+165}{2}} - q^{\frac{m+167}{2}} + q^{\frac{m+169}{2}} - 2q^{\frac{m+171}{2}} \\
& + q^{\frac{m+173}{2}} - q^{49} + q^{48} - q^{47} + q^{46} + 2q^{45} - 2q^{44} + 2q^{43} - q^{42} + 2q^{41} - 2q^{40} + q^{39} \\
t_{19}(q, q^m) = & q^{\frac{m}{2}+24} \left( -2q^{\frac{m}{2}+66} - q^{\frac{m}{2}+67} - 4q^{\frac{m}{2}+68} - q^{\frac{m}{2}+69} - 3q^{\frac{m}{2}+70} - q^{\frac{m}{2}+71} - 3q^{\frac{m}{2}+72} - 2q^{\frac{m}{2}+73} \right. \\
& - 7q^{\frac{m}{2}+74} - 7q^{\frac{m}{2}+75} - 3q^{\frac{m}{2}+76} - 3q^{\frac{m}{2}+77} - q^{\frac{m}{2}+78} - 2q^{\frac{m}{2}+79} - q^{\frac{m}{2}+80} - 3q^{\frac{m}{2}+81} \\
& - 2q^{\frac{m}{2}+82} - q^{\frac{m}{2}+84} + q^{\frac{m}{2}+85} - q^{m+\frac{197}{2}} + q^{m+\frac{199}{2}} + 2q^{m+\frac{203}{2}} + 3q^{m+\frac{205}{2}} + q^{m+\frac{207}{2}} \\
& + 2q^{m+\frac{209}{2}} + q^{m+\frac{211}{2}} + 3q^{m+\frac{213}{2}} + 3q^{m+\frac{215}{2}} + 7q^{m+\frac{217}{2}} + 7q^{m+\frac{219}{2}} + 2q^{m+\frac{221}{2}} + 3q^{m+\frac{223}{2}} \\
& + q^{m+\frac{225}{2}} + 3q^{m+\frac{227}{2}} + q^{m+\frac{229}{2}} + 4q^{m+\frac{231}{2}} + q^{m+\frac{233}{2}} + 2q^{m+\frac{235}{2}} - q^{\frac{3m}{2}+148} + q^{\frac{3m}{2}+149} \\
& \left. - 2q^{\frac{3m}{2}+150} + q^{71/2} - q^{69/2} + 2q^{67/2} \right) \\
t_{20}(q, q^m) = & q^{m+84} + 2q^{m+86} + 2q^{m+88} + 4q^{m+89} + 3q^{m+90} + 5q^{m+91} + 3q^{m+92} + 8q^{m+93} + 6q^{m+94} \\
& + 11q^{m+95} + 9q^{m+96} + 11q^{m+97} + 6q^{m+98} + 6q^{m+99} + 11q^{m+100} + 9q^{m+101} + 11q^{m+102} \\
& + 6q^{m+103} + 8q^{m+104} + 3q^{m+105} + 5q^{m+106} + 3q^{m+107} + 4q^{m+108} + 2q^{m+109} \\
& + 2q^{m+111} + q^{m+113} - q^{\frac{3m}{2}+\frac{235}{2}} - 2q^{\frac{3m}{2}+\frac{239}{2}} - 2q^{\frac{3m}{2}+\frac{253}{2}} - q^{\frac{3m}{2}+\frac{257}{2}} + q^{\frac{3(m+79)}{2}} \\
& - 3q^{\frac{3(m+81)}{2}} - 3q^{\frac{3(m+83)}{2}} + q^{\frac{3(m+85)}{2}} - q^{\frac{m+119}{2}} - 2q^{\frac{m+123}{2}} - 2q^{\frac{m+127}{2}} - 4q^{\frac{m+129}{2}} - 3q^{\frac{m+131}{2}} \\
& - 5q^{\frac{m+133}{2}} - 3q^{\frac{m+135}{2}} - 8q^{\frac{m+137}{2}} - 6q^{\frac{m+139}{2}} - 11q^{\frac{m+141}{2}} - 9q^{\frac{m+143}{2}} - 11q^{\frac{m+145}{2}} \\
& - 6q^{\frac{m+147}{2}} - 6q^{\frac{m+149}{2}} - 11q^{\frac{m+151}{2}} - 9q^{\frac{m+153}{2}} - 11q^{\frac{m+155}{2}} - 6q^{\frac{m+157}{2}} - 8q^{\frac{m+159}{2}} - 3q^{\frac{m+161}{2}} \\
& - 5q^{\frac{m+163}{2}} - 3q^{\frac{m+165}{2}} - 4q^{\frac{m+167}{2}} - 2q^{\frac{m+169}{2}} - 2q^{\frac{m+173}{2}} - q^{\frac{m+177}{2}} + q^{55} - q^{54} + 2q^{53} + 3q^{51} \\
& + 3q^{48} + 2q^{46} - q^{45} + q^{44} \\
t_{21}(q, q^m) = & q^{\frac{m}{2}+18} \left( -q^{\frac{m}{2}+69} - q^{\frac{m}{2}+70} - 2q^{\frac{m}{2}+71} - q^{\frac{m}{2}+72} - 3q^{\frac{m}{2}+73} + q^{\frac{m}{2}+74} - 4q^{\frac{m}{2}+75} - q^{\frac{m}{2}+76} \right. \\
& - 6q^{\frac{m}{2}+77} - 3q^{\frac{m}{2}+78} - 4q^{\frac{m}{2}+79} + q^{\frac{m}{2}+80} - q^{\frac{m}{2}+81} - 2q^{\frac{m}{2}+82} - 3q^{\frac{m}{2}+83} - 4q^{\frac{m}{2}+84} \\
& - 3q^{\frac{m}{2}+85} - 3q^{\frac{m}{2}+86} - q^{\frac{m}{2}+88} - 3q^{\frac{m}{2}+89} - q^{\frac{m}{2}+90} - 2q^{\frac{m}{2}+91} + q^{\frac{m}{2}+92} - q^{\frac{m}{2}+93} + q^{m+\frac{201}{2}} \\
& - q^{m+\frac{203}{2}} + 2q^{m+\frac{205}{2}} + q^{m+\frac{207}{2}} + 3q^{m+\frac{209}{2}} + q^{m+\frac{211}{2}} + 3q^{m+\frac{215}{2}} + 3q^{m+\frac{217}{2}} + 4q^{m+\frac{219}{2}} \\
& + 3q^{m+\frac{221}{2}} + 2q^{m+\frac{223}{2}} + q^{m+\frac{225}{2}} - q^{m+\frac{227}{2}} + 4q^{m+\frac{229}{2}} + 3q^{m+\frac{231}{2}} + 6q^{m+\frac{233}{2}} + q^{m+\frac{235}{2}} \\
& + 4q^{m+\frac{237}{2}} - q^{m+\frac{239}{2}} + 3q^{m+\frac{241}{2}} + q^{m+\frac{243}{2}} + 2q^{m+\frac{245}{2}} + q^{m+\frac{247}{2}} + q^{m+\frac{249}{2}} - q^{\frac{3m}{2}+148} \\
& - q^{\frac{3m}{2}+149} + 2q^{\frac{3m}{2}+150} - 2q^{\frac{3m}{2}+151} + q^{\frac{3m}{2}+152} - q^{\frac{3m}{2}+153} + q^{93/2} + q^{91/2} + q^{89/2} \\
& \left. - 2q^{87/2} + 2q^{85/2} - q^{83/2} + q^{81/2} - q^{\frac{3(m+98)}{2}} \right) \\
t_{22}(q, q^m) = & q^{m+85} - q^{m+86} + q^{m+88} - q^{m+89} + q^{m+90} + 5q^{m+92} - q^{m+93} + 4q^{m+94} - 2q^{m+95} \\
& + 3q^{m+96} + q^{m+97} + 7q^{m+98} + 6q^{m+99} + 2q^{m+100} + 2q^{m+103} + 2q^{m+105} + q^{m+106} \\
& + q^{m+107} - q^{m+109} + q^{m+110} - q^{m+111} + 2q^{m+112} - q^{m+113} - q^{\frac{3m}{2}+\frac{229}{2}} - 2q^{\frac{3m}{2}+\frac{233}{2}} \\
& + q^{\frac{3m}{2}+\frac{235}{2}} + 2q^{\frac{3m}{2}+\frac{239}{2}} - 2q^{\frac{3m}{2}+\frac{241}{2}} + q^{\frac{3m}{2}+\frac{245}{2}} - q^{\frac{3m}{2}+\frac{247}{2}} + 2q^{\frac{3(m+77)}{2}} - 2q^{\frac{3(m+79)}{2}} \\
& - q^{\frac{3(m+81)}{2}} + q^{\frac{3(m+83)}{2}} + q^{\frac{m+123}{2}} - 2q^{\frac{m+125}{2}} + q^{\frac{m+127}{2}} - q^{\frac{m+129}{2}} + q^{\frac{m+131}{2}} - q^{\frac{m+135}{2}}
\end{aligned}$$

$$\begin{aligned}
& -q^{\frac{m+137}{2}} - 2q^{\frac{m+139}{2}} - 2q^{\frac{m+143}{2}} - 2q^{\frac{m+149}{2}} - 6q^{\frac{m+151}{2}} - 7q^{\frac{m+153}{2}} - q^{\frac{m+155}{2}} - 3q^{\frac{m+157}{2}} \\
& + 2q^{\frac{m+159}{2}} - 4q^{\frac{m+161}{2}} + q^{\frac{m+163}{2}} - 5q^{\frac{m+165}{2}} - q^{\frac{m+169}{2}} + q^{\frac{m+171}{2}} - q^{\frac{m+173}{2}} + q^{\frac{m+177}{2}} \\
& - q^{\frac{m+179}{2}} + q^{60} - 2q^{59} + 2q^{58} - q^{57} + 2q^{56} - 2q^{55} + 2q^{54} + q^{53} - q^{52} + q^{51} - q^{50} \\
t_{23}(q, q^m) = & q^{\frac{m}{2}+13} \left( q^{\frac{m}{2}+74} + 2q^{\frac{m}{2}+76} + 3q^{\frac{m}{2}+78} - q^{\frac{m}{2}+79} + 5q^{\frac{m}{2}+80} + 2q^{\frac{m}{2}+81} + 9q^{\frac{m}{2}+82} + 4q^{\frac{m}{2}+83} \right. \\
& + 8q^{\frac{m}{2}+84} + q^{\frac{m}{2}+85} + 3q^{\frac{m}{2}+86} + 4q^{\frac{m}{2}+87} + 7q^{\frac{m}{2}+88} + 5q^{\frac{m}{2}+89} + 4q^{\frac{m}{2}+90} + 3q^{\frac{m}{2}+91} \\
& + q^{\frac{m}{2}+93} + 3q^{\frac{m}{2}+94} - q^{\frac{m}{2}+95} + q^{\frac{m}{2}+96} - q^{\frac{m}{2}+97} + 2q^{\frac{m}{2}+98} - q^{\frac{m}{2}+99} + q^{m+\frac{205}{2}} - 2q^{m+\frac{207}{2}} \\
& + q^{m+\frac{209}{2}} - q^{m+\frac{211}{2}} + q^{m+\frac{213}{2}} - 3q^{m+\frac{215}{2}} - q^{m+\frac{217}{2}} - 3q^{m+\frac{221}{2}} - 4q^{m+\frac{223}{2}} - 5q^{m+\frac{225}{2}} \\
& - 7q^{m+\frac{227}{2}} - 4q^{m+\frac{229}{2}} - 3q^{m+\frac{231}{2}} - q^{m+\frac{233}{2}} - 8q^{m+\frac{235}{2}} - 4q^{m+\frac{237}{2}} - 9q^{m+\frac{239}{2}} - 2q^{m+\frac{241}{2}} \\
& - 5q^{m+\frac{243}{2}} + q^{m+\frac{245}{2}} - 3q^{m+\frac{247}{2}} - 2q^{m+\frac{251}{2}} - q^{m+\frac{255}{2}} + 2q^{\frac{3m}{2}+148} + q^{\frac{3m}{2}+149} + 2q^{\frac{3m}{2}+150} \\
& - 2q^{\frac{3m}{2}+151} + 3q^{\frac{3m}{2}+152} - 2q^{\frac{3m}{2}+153} + q^{\frac{3m}{2}+154} + q^{109/2} - 2q^{107/2} - q^{105/2} - 2q^{103/2} \\
& \left. + 2q^{101/2} - 3q^{99/2} + 2q^{97/2} - q^{95/2} - q^{\frac{3(m+98)}{2}} \right) \\
t_{24}(q, q^m) = & -q^{m+85} - q^{m+86} - q^{m+87} - 2q^{m+88} - q^{m+89} - 4q^{m+90} - 2q^{m+91} - 8q^{m+92} - 3q^{m+93} \\
& - 8q^{m+94} - 2q^{m+95} - 7q^{m+96} - 4q^{m+97} - 11q^{m+98} - 9q^{m+99} - 7q^{m+100} - 4q^{m+101} \\
& - 5q^{m+102} - 6q^{m+103} - 5q^{m+104} - 5q^{m+105} - 3q^{m+106} - 3q^{m+107} - 3q^{m+108} - 2q^{m+110} \\
& + q^{m+111} - 2q^{m+112} - 2q^{\frac{3m}{2}+\frac{227}{2}} + 3q^{\frac{3m}{2}+\frac{229}{2}} + 2q^{\frac{3m}{2}+\frac{233}{2}} - q^{\frac{3m}{2}+\frac{235}{2}} + q^{\frac{3m}{2}+\frac{239}{2}} \\
& + 2q^{\frac{3(m+75)}{2}} - q^{\frac{3(m+77)}{2}} + 2q^{\frac{3(m+79)}{2}} + q^{\frac{3(m+81)}{2}} + 2q^{\frac{m+129}{2}} - q^{\frac{m+131}{2}} + 2q^{\frac{m+133}{2}} + 3q^{\frac{m+137}{2}} \\
& + 3q^{\frac{m+139}{2}} + 3q^{\frac{m+141}{2}} + 5q^{\frac{m+143}{2}} + 5q^{\frac{m+145}{2}} + 6q^{\frac{m+147}{2}} + 5q^{\frac{m+149}{2}} + 4q^{\frac{m+151}{2}} + 7q^{\frac{m+153}{2}} \\
& + 9q^{\frac{m+155}{2}} + 11q^{\frac{m+157}{2}} + 4q^{\frac{m+159}{2}} + 7q^{\frac{m+161}{2}} + 2q^{\frac{m+163}{2}} + 8q^{\frac{m+165}{2}} + 3q^{\frac{m+167}{2}} + 8q^{\frac{m+169}{2}} \\
& + 2q^{\frac{m+171}{2}} + 4q^{\frac{m+173}{2}} + q^{\frac{m+175}{2}} + 2q^{\frac{m+177}{2}} + q^{\frac{m+179}{2}} + q^{\frac{m+181}{2}} + q^{\frac{m+183}{2}} - 2q^{64} + 2q^{63} \\
& - 3q^{62} + q^{61} - 2q^{60} + q^{59} - 2q^{58} - q^{57} - q^{55} \\
t_{25}(q, q^m) = & q^{\frac{m}{2}+6} \left( q^{\frac{m}{2}+79} + q^{\frac{m}{2}+80} + q^{\frac{m}{2}+81} + 2q^{\frac{m}{2}+82} + q^{\frac{m}{2}+83} + 4q^{\frac{m}{2}+84} + 2q^{\frac{m}{2}+85} + 8q^{\frac{m}{2}+86} \right. \\
& + 3q^{\frac{m}{2}+87} + 8q^{\frac{m}{2}+88} + 2q^{\frac{m}{2}+89} + 7q^{\frac{m}{2}+90} + 4q^{\frac{m}{2}+91} + 11q^{\frac{m}{2}+92} + 9q^{\frac{m}{2}+93} + 7q^{\frac{m}{2}+94} \\
& + 4q^{\frac{m}{2}+95} + 5q^{\frac{m}{2}+96} + 6q^{\frac{m}{2}+97} + 5q^{\frac{m}{2}+98} + 5q^{\frac{m}{2}+99} + 3q^{\frac{m}{2}+100} + 3q^{\frac{m}{2}+101} + 3q^{\frac{m}{2}+102} \\
& + 2q^{\frac{m}{2}+104} - q^{\frac{m}{2}+105} + 2q^{\frac{m}{2}+106} - 2q^{m+\frac{215}{2}} + q^{m+\frac{217}{2}} - 2q^{m+\frac{219}{2}} - 3q^{m+\frac{223}{2}} - 3q^{m+\frac{225}{2}} \\
& - 3q^{m+\frac{227}{2}} - 5q^{m+\frac{229}{2}} - 5q^{m+\frac{231}{2}} - 6q^{m+\frac{233}{2}} - 5q^{m+\frac{235}{2}} - 4q^{m+\frac{237}{2}} - 7q^{m+\frac{239}{2}} - 9q^{m+\frac{241}{2}} \\
& - 11q^{m+\frac{243}{2}} - 4q^{m+\frac{245}{2}} - 7q^{m+\frac{247}{2}} - 2q^{m+\frac{249}{2}} - 8q^{m+\frac{251}{2}} - 3q^{m+\frac{253}{2}} - 8q^{m+\frac{255}{2}} \\
& - 2q^{m+\frac{257}{2}} - 4q^{m+\frac{259}{2}} - q^{m+\frac{261}{2}} - 2q^{m+\frac{263}{2}} - q^{m+\frac{265}{2}} - q^{m+\frac{267}{2}} - q^{m+\frac{269}{2}} + q^{\frac{3m}{2}+149} \\
& + 2q^{\frac{3m}{2}+150} - q^{\frac{3m}{2}+151} + 2q^{\frac{3m}{2}+152} - q^{\frac{3m}{2}+153} + 3q^{\frac{3m}{2}+154} - 2q^{\frac{3m}{2}+155} + 2q^{\frac{3m}{2}+156} \\
& - q^{133/2} - q^{129/2} - 2q^{127/2} + q^{125/2} - 2q^{123/2} + q^{121/2} - 3q^{119/2} + 2q^{117/2} - 2q^{115/2} \\
& \left. + q^{\frac{3(m+98)}{2}} \right) \\
t_{26}(q, q^m) = & q^{123/2} \left( -q^{\frac{m}{2}+5} + 2q^{\frac{m}{2}+6} - q^{\frac{m}{2}+7} + q^{\frac{m}{2}+8} - q^{\frac{m}{2}+9} + 3q^{\frac{m}{2}+10} + q^{\frac{m}{2}+11} + 3q^{\frac{m}{2}+13} \right)
\end{aligned}$$

$$\begin{aligned}
& + 4q^{\frac{m}{2}+14} + 5q^{\frac{m}{2}+15} + 7q^{\frac{m}{2}+16} + 4q^{\frac{m}{2}+17} + 3q^{\frac{m}{2}+18} + q^{\frac{m}{2}+19} + 8q^{\frac{m}{2}+20} + 4q^{\frac{m}{2}+21} \\
& + 9q^{\frac{m}{2}+22} + 2q^{\frac{m}{2}+23} + 5q^{\frac{m}{2}+24} - q^{\frac{m}{2}+25} + 3q^{\frac{m}{2}+26} + 2q^{\frac{m}{2}+28} + q^{\frac{m}{2}+30} - q^{m+\frac{51}{2}} \\
& - 2q^{m+\frac{55}{2}} - 3q^{m+\frac{59}{2}} + q^{m+\frac{61}{2}} - 5q^{m+\frac{63}{2}} - 2q^{m+\frac{65}{2}} - 9q^{m+\frac{67}{2}} - 4q^{m+\frac{69}{2}} - 8q^{m+\frac{71}{2}} \\
& - q^{m+\frac{73}{2}} - 3q^{m+\frac{75}{2}} - 4q^{m+\frac{77}{2}} - 7q^{m+\frac{79}{2}} - 5q^{m+\frac{81}{2}} - 4q^{m+\frac{83}{2}} - 3q^{m+\frac{85}{2}} - q^{m+\frac{89}{2}} \\
& - 3q^{m+\frac{91}{2}} + q^{m+\frac{93}{2}} - q^{m+\frac{95}{2}} + q^{m+\frac{97}{2}} - 2q^{m+\frac{99}{2}} + q^{m+\frac{101}{2}} + q^{\frac{3m}{2}+48} - 2q^{\frac{3m}{2}+49} \\
& + 3q^{\frac{3m}{2}+50} - 2q^{\frac{3m}{2}+51} + 2q^{\frac{3m}{2}+52} + q^{\frac{3m}{2}+53} + 2q^{\frac{3m}{2}+54} - q^{\frac{3m}{2}+55} - q^{15/2} + 2q^{13/2} \\
& - 3q^{11/2} + 2q^{9/2} - 2q^{7/2} - q^{5/2} - 2q^{3/2} + \sqrt{q} \Big) \\
t_{27}(q, q^m) &= q^{\frac{m}{2}+1} \Big( -q^{\frac{m}{2}+84} + q^{\frac{m}{2}+85} - q^{\frac{m}{2}+87} + q^{\frac{m}{2}+88} - q^{\frac{m}{2}+89} - 5q^{\frac{m}{2}+91} + q^{\frac{m}{2}+92} - 4q^{\frac{m}{2}+93} \\
& + 2q^{\frac{m}{2}+94} - 3q^{\frac{m}{2}+95} - q^{\frac{m}{2}+96} - 7q^{\frac{m}{2}+97} - 6q^{\frac{m}{2}+98} - 2q^{\frac{m}{2}+99} - 2q^{\frac{m}{2}+102} - 2q^{\frac{m}{2}+104} \\
& - q^{\frac{m}{2}+105} - q^{\frac{m}{2}+106} + q^{\frac{m}{2}+108} - q^{\frac{m}{2}+109} + q^{\frac{m}{2}+110} - 2q^{\frac{m}{2}+111} + q^{\frac{m}{2}+112} - q^{m+\frac{219}{2}} \\
& + 2q^{m+\frac{221}{2}} - q^{m+\frac{223}{2}} + q^{m+\frac{225}{2}} - q^{m+\frac{227}{2}} + q^{m+\frac{231}{2}} + q^{m+\frac{233}{2}} + 2q^{m+\frac{235}{2}} + 2q^{m+\frac{239}{2}} \\
& + 2q^{m+\frac{245}{2}} + 6q^{m+\frac{247}{2}} + 7q^{m+\frac{249}{2}} + q^{m+\frac{251}{2}} + 3q^{m+\frac{253}{2}} - 2q^{m+\frac{255}{2}} + 4q^{m+\frac{257}{2}} - q^{m+\frac{259}{2}} \\
& + 5q^{m+\frac{261}{2}} + q^{m+\frac{265}{2}} - q^{m+\frac{267}{2}} + q^{m+\frac{269}{2}} - q^{m+\frac{273}{2}} + q^{m+\frac{275}{2}} - q^{\frac{3m}{2}+148} + q^{\frac{3m}{2}+149} \\
& - q^{\frac{3m}{2}+150} - 2q^{\frac{3m}{2}+151} + 2q^{\frac{3m}{2}+152} - 2q^{\frac{3m}{2}+153} + q^{\frac{3m}{2}+154} - 2q^{\frac{3m}{2}+155} + 2q^{\frac{3m}{2}+156} \\
& - q^{\frac{3m}{2}+157} - q^{149/2} + q^{147/2} - q^{145/2} + q^{143/2} + 2q^{141/2} - 2q^{139/2} + 2q^{137/2} - q^{135/2} \\
& + 2q^{133/2} - 2q^{131/2} + q^{129/2} + q^{\frac{3(m+98)}{2}} \Big) \\
t_{28}(q, q^m) &= q^{133/2} \Big( -q^{\frac{m}{2}+3} + q^{\frac{m}{2}+4} - 2q^{\frac{m}{2}+5} - q^{\frac{m}{2}+6} - 3q^{\frac{m}{2}+7} - q^{\frac{m}{2}+8} - 3q^{\frac{m}{2}+10} - 3q^{\frac{m}{2}+11} \\
& - 4q^{\frac{m}{2}+12} - 3q^{\frac{m}{2}+13} - 2q^{\frac{m}{2}+14} - q^{\frac{m}{2}+15} + q^{\frac{m}{2}+16} - 4q^{\frac{m}{2}+17} - 3q^{\frac{m}{2}+18} - 6q^{\frac{m}{2}+19} \\
& - q^{\frac{m}{2}+20} - 4q^{\frac{m}{2}+21} + q^{\frac{m}{2}+22} - 3q^{\frac{m}{2}+23} - q^{\frac{m}{2}+24} - 2q^{\frac{m}{2}+25} - q^{\frac{m}{2}+26} - q^{\frac{m}{2}+27} \\
& + q^{m+\frac{41}{2}} + q^{m+\frac{43}{2}} + 2q^{m+\frac{45}{2}} + q^{m+\frac{47}{2}} + 3q^{m+\frac{49}{2}} - q^{m+\frac{51}{2}} + 4q^{m+\frac{53}{2}} + q^{m+\frac{55}{2}} \\
& + 6q^{m+\frac{57}{2}} + 3q^{m+\frac{59}{2}} + 4q^{m+\frac{61}{2}} - q^{m+\frac{63}{2}} + q^{m+\frac{65}{2}} + 2q^{m+\frac{67}{2}} + 3q^{m+\frac{69}{2}} + 4q^{m+\frac{71}{2}} \\
& + 3q^{m+\frac{73}{2}} + 3q^{m+\frac{75}{2}} + q^{m+\frac{79}{2}} + 3q^{m+\frac{81}{2}} + q^{m+\frac{83}{2}} + 2q^{m+\frac{85}{2}} - q^{m+\frac{87}{2}} + q^{m+\frac{89}{2}} - q^{\frac{3m}{2}+41} \\
& + q^{\frac{3m}{2}+42} - 2q^{\frac{3m}{2}+43} + 2q^{\frac{3m}{2}+44} - q^{\frac{3m}{2}+45} - q^{\frac{3m}{2}+46} - q^{\frac{3m}{2}+47} + q^{13/2} - q^{11/2} \\
& + 2q^{9/2} - 2q^{7/2} + q^{5/2} + q^{3/2} + \sqrt{q} \Big) \\
t_{29}(q, q^m) &= -q^{\frac{m+137}{2}} \Big( -q^{m+40} - 2q^{m+42} - 2q^{m+44} - 4q^{m+45} - 3q^{m+46} - 5q^{m+47} - 3q^{m+48} \\
& - 8q^{m+49} - 6q^{m+50} - 11q^{m+51} - 9q^{m+52} - 11q^{m+53} - 6q^{m+54} - 6q^{m+55} - 11q^{m+56} \\
& - 9q^{m+57} - 11q^{m+58} - 6q^{m+59} - 8q^{m+60} - 3q^{m+61} - 5q^{m+62} - 3q^{m+63} - 4q^{m+64} \\
& - 2q^{m+65} - 2q^{m+67} - q^{m+69} - q^{\frac{3m}{2}+\frac{149}{2}} + 2q^{\frac{3m}{2}+\frac{151}{2}} + 3q^{\frac{3m}{2}+\frac{155}{2}} + 3q^{\frac{3m}{2}+\frac{161}{2}} \\
& - q^{\frac{3m}{2}+\frac{167}{2}} + q^{\frac{3m}{2}+\frac{169}{2}} + q^{\frac{m+31}{2}} + 2q^{\frac{m+35}{2}} + 2q^{\frac{m+39}{2}} + 4q^{\frac{m+41}{2}} + 3q^{\frac{m+43}{2}} + 5q^{\frac{m+45}{2}} \\
& + 3q^{\frac{m+47}{2}} + 8q^{\frac{m+49}{2}} + q^{\frac{3(m+49)}{2}} + 6q^{\frac{m+51}{2}} + 11q^{\frac{m+53}{2}} + 9q^{\frac{m+55}{2}} + 2q^{\frac{3(m+55)}{2}} + 11q^{\frac{m+57}{2}} \Big)
\end{aligned}$$

$$\begin{aligned}
& + 6q^{\frac{m+59}{2}} + 6q^{\frac{m+61}{2}} + 11q^{\frac{m+63}{2}} + 9q^{\frac{m+65}{2}} + 11q^{\frac{m+67}{2}} + 6q^{\frac{m+69}{2}} + 8q^{\frac{m+71}{2}} + 3q^{\frac{m+73}{2}} \\
& + 5q^{\frac{m+75}{2}} + 3q^{\frac{m+77}{2}} + 4q^{\frac{m+79}{2}} + 2q^{\frac{m+81}{2}} + 2q^{\frac{m+85}{2}} + q^{\frac{m+89}{2}} - q^{11} + q^{10} - 2q^9 - 3q^7 \\
& - 3q^4 - 2q^2 + q - 1)
\end{aligned}$$

$$\begin{aligned}
t_{30}(q, q^m) = & q^{147/2} \left( -q^{\frac{m}{2}+1} - 2q^{\frac{m}{2}+3} - 3q^{\frac{m}{2}+4} - q^{\frac{m}{2}+5} - 2q^{\frac{m}{2}+6} - q^{\frac{m}{2}+7} - 3q^{\frac{m}{2}+8} - 3q^{\frac{m}{2}+9} \right. \\
& - 7q^{\frac{m}{2}+10} - 7q^{\frac{m}{2}+11} - 2q^{\frac{m}{2}+12} - 3q^{\frac{m}{2}+13} - q^{\frac{m}{2}+14} - 3q^{\frac{m}{2}+15} - q^{\frac{m}{2}+16} - 4q^{\frac{m}{2}+17} \\
& - q^{\frac{m}{2}+18} - 2q^{\frac{m}{2}+19} + q^{m/2} + 2q^{m+\frac{33}{2}} + q^{m+\frac{35}{2}} + 4q^{m+\frac{37}{2}} + q^{m+\frac{39}{2}} + 3q^{m+\frac{41}{2}} + q^{m+\frac{43}{2}} \\
& + 3q^{m+\frac{45}{2}} + 2q^{m+\frac{47}{2}} + 7q^{m+\frac{49}{2}} + 7q^{m+\frac{51}{2}} + 3q^{m+\frac{53}{2}} + 3q^{m+\frac{55}{2}} + q^{m+\frac{57}{2}} + 2q^{m+\frac{59}{2}} \\
& + q^{m+\frac{61}{2}} + 3q^{m+\frac{63}{2}} + 2q^{m+\frac{65}{2}} + q^{m+\frac{69}{2}} - q^{m+\frac{71}{2}} - 2q^{\frac{3m}{2}+33} + q^{\frac{3m}{2}+34} - q^{\frac{3m}{2}+35} + 2q^{5/2} \\
& \left. - q^{3/2} + \sqrt{q} \right)
\end{aligned}$$

$$\begin{aligned}
t_{31}(q, q^m) = & q^{\frac{m+145}{2}} \left( q^{m+35} - q^{m+36} + q^{m+38} - q^{m+39} + q^{m+40} + 5q^{m+42} - q^{m+43} + 4q^{m+44} - 2q^{m+45} \right. \\
& + 3q^{m+46} + q^{m+47} + 7q^{m+48} + 6q^{m+49} + 2q^{m+50} + 2q^{m+53} + 2q^{m+55} + q^{m+56} + q^{m+57} \\
& - q^{m+59} + q^{m+60} - q^{m+61} + 2q^{m+62} - q^{m+63} + 2q^{\frac{3m}{2}+\frac{131}{2}} - 2q^{\frac{3m}{2}+\frac{133}{2}} - 2q^{\frac{3m}{2}+\frac{137}{2}} \\
& + 2q^{\frac{3m}{2}+\frac{139}{2}} - q^{\frac{3m}{2}+\frac{143}{2}} + q^{\frac{3m}{2}+\frac{145}{2}} + q^{\frac{3m}{2}+\frac{149}{2}} + q^{\frac{m+23}{2}} - 2q^{\frac{m+25}{2}} + q^{\frac{m+27}{2}} - q^{\frac{m+29}{2}} \\
& + q^{\frac{m+31}{2}} - q^{\frac{m+35}{2}} - q^{\frac{m+37}{2}} - 2q^{\frac{m+39}{2}} - 2q^{\frac{m+43}{2}} - q^{\frac{3(m+43)}{2}} + q^{\frac{3(m+45)}{2}} - 2q^{\frac{3(m+47)}{2}} \\
& - 2q^{\frac{m+49}{2}} - q^{\frac{3(m+49)}{2}} - 6q^{\frac{m+51}{2}} - 7q^{\frac{m+53}{2}} - q^{\frac{m+55}{2}} - 3q^{\frac{m+57}{2}} + 2q^{\frac{m+59}{2}} - 4q^{\frac{m+61}{2}} + q^{\frac{m+63}{2}} \\
& - 5q^{\frac{m+65}{2}} - q^{\frac{m+69}{2}} + q^{\frac{m+71}{2}} - q^{\frac{m+73}{2}} + q^{\frac{m+77}{2}} - q^{\frac{m+79}{2}} + q^{10} - 2q^9 + 2q^8 - q^7 + 2q^6 \\
& \left. - 2q^5 + 2q^4 + q^3 - q^2 + q - 1 \right)
\end{aligned}$$

$$\begin{aligned}
t_{32}(q, q^m) = & -q^{m+90} - q^{m+91} - 2q^{m+92} + q^{m+97} - 2q^{m+98} - 3q^{m+99} - q^{m+101} + 3q^{m+102} - q^{m+103} \\
& - 2q^{m+105} - q^{m+106} - q^{m+108} + q^{\frac{3m}{2}+\frac{209}{2}} + q^{\frac{m+153}{2}} + q^{\frac{m+157}{2}} + 2q^{\frac{m+159}{2}} + q^{\frac{m+163}{2}} \\
& - 3q^{\frac{m+165}{2}} + q^{\frac{m+167}{2}} + 3q^{\frac{m+171}{2}} + 2q^{\frac{m+173}{2}} - q^{\frac{m+175}{2}} + 2q^{\frac{m+185}{2}} + q^{\frac{m+187}{2}} + q^{\frac{m+189}{2}} - q^{80}
\end{aligned}$$

$$\begin{aligned}
t_{33}(q, q^m) = & q^{\frac{m+151}{2}} \left( -q^{m+30} - q^{m+31} - q^{m+32} - 2q^{m+33} - q^{m+34} - 4q^{m+35} - 2q^{m+36} - 8q^{m+37} \right. \\
& - 3q^{m+38} - 8q^{m+39} - 2q^{m+40} - 7q^{m+41} - 4q^{m+42} - 11q^{m+43} - 9q^{m+44} - 7q^{m+45} \\
& - 4q^{m+46} - 5q^{m+47} - 6q^{m+48} - 5q^{m+49} - 5q^{m+50} - 3q^{m+51} - 3q^{m+52} - 3q^{m+53} \\
& - 2q^{m+55} + q^{m+56} - 2q^{m+57} + 2q^{\frac{3m}{2}+\frac{115}{2}} + 3q^{\frac{3m}{2}+\frac{119}{2}} - q^{\frac{3m}{2}+\frac{121}{2}} - q^{\frac{3m}{2}+\frac{125}{2}} + 2q^{\frac{3m}{2}+\frac{127}{2}} \\
& + q^{\frac{3m}{2}+\frac{133}{2}} + 2q^{\frac{m+19}{2}} - q^{\frac{m+21}{2}} + 2q^{\frac{m+23}{2}} + 3q^{\frac{m+27}{2}} + 3q^{\frac{m+29}{2}} + 3q^{\frac{m+31}{2}} + 5q^{\frac{m+33}{2}} \\
& + 5q^{\frac{m+35}{2}} + 6q^{\frac{m+37}{2}} + 5q^{\frac{m+39}{2}} - 2q^{\frac{3(m+39)}{2}} + 4q^{\frac{m+41}{2}} + 2q^{\frac{3(m+41)}{2}} + 7q^{\frac{m+43}{2}} + q^{\frac{3(m+43)}{2}} \\
& + 9q^{\frac{m+45}{2}} + 11q^{\frac{m+47}{2}} + 4q^{\frac{m+49}{2}} + 7q^{\frac{m+51}{2}} + 2q^{\frac{m+53}{2}} + 8q^{\frac{m+55}{2}} + 3q^{\frac{m+57}{2}} + 8q^{\frac{m+59}{2}} \\
& + 2q^{\frac{m+61}{2}} + 4q^{\frac{m+63}{2}} + q^{\frac{m+65}{2}} + 2q^{\frac{m+67}{2}} + q^{\frac{m+69}{2}} + q^{\frac{m+71}{2}} + q^{\frac{m+73}{2}} - 2q^9 + 2q^8 - 3q^7 \\
& \left. + q^6 - 2q^5 + q^4 - 2q^3 - q^2 - 1 \right)
\end{aligned}$$

$$\begin{aligned}
t_{34}(q, q^m) &= q^{\frac{m+163}{2}} \left( -q^{\frac{m+23}{2}} - 3q^{\frac{m+25}{2}} - 2q^{\frac{m+27}{2}} - q^{\frac{m+29}{2}} - 2q^{\frac{m+31}{2}} - q^{\frac{m+33}{2}} + q^{\frac{m+35}{2}} - 2q^{\frac{m+37}{2}} \right. \\
&\quad - 4q^{\frac{m+41}{2}} - 2q^{\frac{m+43}{2}} - 2q^{\frac{m+45}{2}} + q^{\frac{m+47}{2}} + q^{12} + 3q^{11} + 2q^{10} + q^9 + 2q^8 + q^7 - q^6 + 2q^5 \\
&\quad \left. + 4q^3 + 2q^2 + 2q - 1 \right) \\
t_{35}(q, q^m) &= -q^{\frac{m+161}{2}} \left( q^{m+25} + 2q^{m+27} + 3q^{m+29} - q^{m+30} + 5q^{m+31} + 2q^{m+32} + 9q^{m+33} + 4q^{m+34} \right. \\
&\quad + 8q^{m+35} + q^{m+36} + 3q^{m+37} + 4q^{m+38} + 7q^{m+39} + 5q^{m+40} + 4q^{m+41} + 3q^{m+42} \\
&\quad + q^{m+44} + 3q^{m+45} - q^{m+46} + q^{m+47} - q^{m+48} + 2q^{m+49} - q^{m+50} - q^{\frac{3m}{2} + \frac{95}{2}} + 2q^{\frac{3m}{2} + \frac{97}{2}} \\
&\quad + 2q^{\frac{3m}{2} + \frac{101}{2}} - 2q^{\frac{3m}{2} + \frac{103}{2}} - 2q^{\frac{3m}{2} + \frac{107}{2}} + q^{\frac{3m}{2} + \frac{109}{2}} + q^{\frac{m+9}{2}} - 2q^{\frac{m+11}{2}} + q^{\frac{m+13}{2}} - q^{\frac{m+15}{2}} \\
&\quad + q^{\frac{m+17}{2}} - 3q^{\frac{m+19}{2}} - q^{\frac{m+21}{2}} - 3q^{\frac{m+25}{2}} - 4q^{\frac{m+27}{2}} - 5q^{\frac{m+29}{2}} - 7q^{\frac{m+31}{2}} - 4q^{\frac{m+33}{2}} - 3q^{\frac{3(m+33)}{2}} \\
&\quad - 3q^{\frac{m+35}{2}} - q^{\frac{3(m+35)}{2}} - q^{\frac{m+37}{2}} - 8q^{\frac{m+39}{2}} - 4q^{\frac{m+41}{2}} - 9q^{\frac{m+43}{2}} - 2q^{\frac{m+45}{2}} - 5q^{\frac{m+47}{2}} \\
&\quad \left. + q^{\frac{m+49}{2}} - 3q^{\frac{m+51}{2}} - 2q^{\frac{m+55}{2}} - q^{\frac{m+59}{2}} + q^7 - 2q^6 + 3q^5 - 2q^4 + 2q^3 + q^2 + 2q - 1 \right) \\
t_{36}(q, q^m) &= q^{\frac{m+169}{2}} \left( q^{\frac{m+19}{2}} + q^{\frac{m+21}{2}} - q^{\frac{m+25}{2}} - q^{\frac{m+29}{2}} + q^{\frac{m+31}{2}} - 2q^{\frac{m+33}{2}} + q^{\frac{m+35}{2}} + q^{\frac{m+37}{2}} + q^{\frac{m+39}{2}} \right. \\
&\quad \left. - q^{10} - q^9 + q^7 + q^5 - q^4 + 2q^3 - q^2 - q - 1 \right) \\
t_{37}(q, q^m) &= -q^{\frac{m+167}{2}} \left( -q^{m+20} - q^{m+21} - 2q^{m+22} - q^{m+23} - 3q^{m+24} + q^{m+25} - 4q^{m+26} - q^{m+27} \right. \\
&\quad - 6q^{m+28} - 3q^{m+29} - 4q^{m+30} + q^{m+31} - q^{m+32} - 2q^{m+33} - 3q^{m+34} - 4q^{m+35} \\
&\quad - 3q^{m+36} - 3q^{m+37} - q^{m+39} - 3q^{m+40} - q^{m+41} - 2q^{m+42} + q^{m+43} - q^{m+44} - q^{\frac{3m}{2} + \frac{83}{2}} \\
&\quad + 2q^{\frac{3m}{2} + \frac{85}{2}} + q^{\frac{3m}{2} + \frac{89}{2}} + q^{\frac{3m}{2} + \frac{91}{2}} + q^{\frac{m+5}{2}} - q^{\frac{m+7}{2}} + 2q^{\frac{m+9}{2}} + q^{\frac{m+11}{2}} + 3q^{\frac{m+13}{2}} + q^{\frac{m+15}{2}} \\
&\quad + 3q^{\frac{m+19}{2}} + 3q^{\frac{m+21}{2}} + 4q^{\frac{m+23}{2}} + 3q^{\frac{m+25}{2}} + 2q^{\frac{m+27}{2}} + q^{\frac{3(m+27)}{2}} + q^{\frac{m+29}{2}} - 2q^{\frac{3(m+29)}{2}} \\
&\quad - q^{\frac{m+31}{2}} + q^{\frac{3(m+31)}{2}} + 4q^{\frac{m+33}{2}} + 3q^{\frac{m+35}{2}} + 6q^{\frac{m+37}{2}} + q^{\frac{m+39}{2}} + 4q^{\frac{m+41}{2}} - q^{\frac{m+43}{2}} + 3q^{\frac{m+45}{2}} \\
&\quad \left. + q^{\frac{m+47}{2}} + 2q^{\frac{m+49}{2}} + q^{\frac{m+51}{2}} + q^{\frac{m+53}{2}} - q^6 + q^5 - 2q^4 + 2q^3 - q^2 - q - 1 \right) \\
t_{38}(q, q^m) &= q^{\frac{m+179}{2}} \left( q^{\frac{m+15}{2}} + q^{\frac{m+17}{2}} + 2q^{\frac{m+19}{2}} - q^{\frac{m+21}{2}} + q^{\frac{m+23}{2}} - q^4 - q^3 - 2q^2 + q - 1 \right) \\
t_{39}(q, q^m) &= q^{\frac{m}{2} + 88} \left( -q^{\frac{m}{2} + 1} - 2q^{\frac{m}{2} + 3} - 3q^{\frac{m}{2} + 4} - q^{\frac{m}{2} + 5} - 2q^{\frac{m}{2} + 6} - q^{\frac{m}{2} + 7} - 3q^{\frac{m}{2} + 8} - 3q^{\frac{m}{2} + 9} \right. \\
&\quad - 7q^{\frac{m}{2} + 10} - 7q^{\frac{m}{2} + 11} - 2q^{\frac{m}{2} + 12} - 3q^{\frac{m}{2} + 13} - q^{\frac{m}{2} + 14} - 3q^{\frac{m}{2} + 15} - q^{\frac{m}{2} + 16} - 4q^{\frac{m}{2} + 17} \\
&\quad - q^{\frac{m}{2} + 18} - 2q^{\frac{m}{2} + 19} + q^{m/2} + 2q^{m+\frac{33}{2}} + q^{m+\frac{35}{2}} + 4q^{m+\frac{37}{2}} + q^{m+\frac{39}{2}} + 3q^{m+\frac{41}{2}} + q^{m+\frac{43}{2}} \\
&\quad + 3q^{m+\frac{45}{2}} + 2q^{m+\frac{47}{2}} + 7q^{m+\frac{49}{2}} + 7q^{m+\frac{51}{2}} + 3q^{m+\frac{53}{2}} + 3q^{m+\frac{55}{2}} + q^{m+\frac{57}{2}} + 2q^{m+\frac{59}{2}} \\
&\quad + q^{m+\frac{61}{2}} + 3q^{m+\frac{63}{2}} + 2q^{m+\frac{65}{2}} + q^{m+\frac{69}{2}} - q^{m+\frac{71}{2}} - 2q^{\frac{3m}{2}+33} + q^{\frac{3m}{2}+34} - q^{\frac{3m}{2}+35} + 2q^{5/2} \\
&\quad \left. - q^{3/2} + \sqrt{q} \right) \\
t_{40}(q, q^m) &= q \left( q^{\frac{m+185}{2}} - q^{m+98} \right) \\
t_{41}(q, q^m) &= q^{177/2} \left( -q^{\frac{m}{2}+4} + q^{m+\frac{1}{2}} + q^{m+\frac{5}{2}} + 2q^{m+\frac{7}{2}} + q^{m+\frac{11}{2}} - 3q^{m+\frac{13}{2}} + q^{m+\frac{15}{2}} + 3q^{m+\frac{19}{2}} \right. \\
&\quad \left. + 2q^{m+\frac{21}{2}} - q^{m+\frac{23}{2}} + 2q^{m+\frac{33}{2}} + q^{m+\frac{35}{2}} + q^{m+\frac{37}{2}} - q^{\frac{3m}{2}+14} - q^{\frac{3m}{2}+15} - 2q^{\frac{3m}{2}+16} \right)
\end{aligned}$$

$$\begin{aligned}
& + q^{\frac{3m}{2}+21} - 2q^{\frac{3m}{2}+22} - 3q^{\frac{3m}{2}+23} - q^{\frac{3m}{2}+25} + 3q^{\frac{3m}{2}+26} - q^{\frac{3m}{2}+27} - 2q^{\frac{3m}{2}+29} - q^{\frac{3m}{2}+30} \\
& - q^{\frac{3m}{2}+32} + q^{2m+\frac{57}{2}} \Big) \\
t_{43}(q, q^m) &= q^{m+54} \Big( -q^{\frac{m+99}{2}} - 3q^{\frac{m+101}{2}} - 2q^{\frac{m+103}{2}} - q^{\frac{m+105}{2}} - 2q^{\frac{m+107}{2}} - q^{\frac{m+109}{2}} + q^{\frac{m+111}{2}} \\
& - 2q^{\frac{m+113}{2}} - 4q^{\frac{m+117}{2}} - 2q^{\frac{m+119}{2}} - 2q^{\frac{m+121}{2}} + q^{\frac{m+123}{2}} + q^{50} + 3q^{49} + 2q^{48} + q^{47} + 2q^{46} \\
& + q^{45} - q^{44} + 2q^{43} + 4q^{41} + 2q^{40} + 2q^{39} - q^{38} \Big) \\
t_{45}(q, q^m) &= q^{m+53} \Big( q^{\frac{m+99}{2}} + q^{\frac{m+101}{2}} - q^{\frac{m+105}{2}} - q^{\frac{m+109}{2}} + q^{\frac{m+111}{2}} - 2q^{\frac{m+113}{2}} + q^{\frac{m+115}{2}} + q^{\frac{m+117}{2}} \\
& + q^{\frac{m+119}{2}} - q^{50} - q^{49} + q^{47} + q^{45} - q^{44} + 2q^{43} - q^{42} - q^{41} - q^{40} \Big) \\
t_{47}(q, q^m) &= q^{m+96} \Big( q^{\frac{m+15}{2}} + q^{\frac{m+17}{2}} + 2q^{\frac{m+19}{2}} - q^{\frac{m+21}{2}} + q^{\frac{m+23}{2}} - q^4 - q^3 - 2q^2 + q - 1 \Big) \\
t_{49}(q, q^m) &= q^{m+98} - q^{\frac{3(m+69)}{2}}.
\end{aligned}$$

## References

- [1] Chae J., A Cable Knot and BPS Series, arXiv (January 2021)
