# Supplementary material for: A Cable Knot and BPS-Series
Source: arXiv:2101.11708 ancillary file (2023-01-18)
Supplement: Supplementary file 3 [file Recursion_Relation_3.pdf]

## The Initial Data for the Recursion Relation

John Chae

Department of Physics and QMAP, UC Davis, 1 Shields Ave, Davis, CA, 95616, USA  
yjchae@ucdavis.edu

We record the initial data  $\{f_m(q) \in \mathbb{Z}[q^{\pm 1}] \mid m = 1, \dots, 97\}$  for the  $f_m$ -recursion relation (9) in Section 4 in [1].

$$\begin{aligned}
 f_1(q) &= f_3(q) = f_5(q) = f_7(q) = f_9(q) = 0 \\
 f_{11}(q) &= q^5 & f_{13}(q) &= 0 & f_{15}(q) &= 2q^6 & f_{17}(q) &= 0 \\
 f_{19}(q) &= q^6 + 3q^7 + q^8 & f_{21}(q) &= 0 \\
 f_{23}(q) &= 2q^6 + 2q^7 + 5q^8 + 2q^9 + 2q^{10} & f_{25}(q) &= 0 \\
 \\
 f_{27}(q) &= q^5 + 3q^6 + 4q^7 + 5q^8 + 8q^9 + 5q^{10} + 4q^{11} + 3q^{12} + q^{13} \\
 f_{29}(q) &= -q^{15} \\
 f_{31}(q) &= 2q^{16} + 2q^{15} + 6q^{14} + 7q^{13} + 10q^{12} + 10q^{11} + 15q^{10} + 10q^9 + 10q^8 + 7q^7 + 6q^6 + 2q^5 + 2q^4 \\
 f_{33}(q) &= -2q^{18} \\
 f_{35}(q) &= q^{20} + 3q^{19} + 4q^{18} + 7q^{17} + 11q^{16} + 15q^{15} + 18q^{14} + 21q^{13} + 23q^{12} + 27q^{11} + 23q^{10} + 21q^9 \\
 &\quad + 18q^8 + 15q^7 + 11q^6 + 7q^5 + 4q^4 + 3q^3 + q^2 \\
 f_{37}(q) &= -q^{22} - 3q^{21} - q^{20} \\
 f_{39}(q) &= 2q^{24} + 2q^{23} + 6q^{22} + 8q^{21} + 13q^{20} + 16q^{19} + 26q^{18} + 29q^{17} + 38q^{16} + 41q^{15} + 48q^{14} \\
 &\quad + 48q^{13} + 56q^{12} + 48q^{11} + 48q^{10} + 41q^9 + 38q^8 + 29q^7 + 26q^6 + 16q^5 + 13q^4 + 8q^3 + 6q^2 \\
 &\quad + 2q + 2 \\
 f_{41}(q) &= -2q^{26} - 2q^{25} - 5q^{24} - 2q^{23} - 2q^{22} \\
 f_{43}(q) &= q^{29} + 3q^{28} + 4q^{27} + 7q^{26} + 13q^{25} + 17q^{24} + 25q^{23} + 33q^{22} + 43q^{21} + 54q^{20} + 67q^{19} + 77q^{18} \\
 &\quad + 88q^{17} + 97q^{16} + 104q^{15} + 108q^{14} + 115q^{13} + 108q^{12} + 104q^{11} + 97q^{10} + 88q^9 + 77q^8 \\
 &\quad + 67q^7 + 54q^6 + 43q^5 + 33q^4 + 25q^3 + 17q^2 + 13q + 7 + \frac{4}{q} + \frac{3}{q^2} + \frac{1}{q^3} \\
 f_{45}(q) &= -q^{31} - 3q^{30} - 4q^{29} - 5q^{28} - 8q^{27} - 5q^{26} - 4q^{25} - 3q^{24} - q^{23} \\
 f_{47}(q) &= 3q^{34} + 2q^{33} + 6q^{32} + 8q^{31} + 14q^{30} + 19q^{29} + 30q^{28} + 38q^{27} + 55q^{26} + 66q^{25} + 87q^{24} \\
 &\quad + 102q^{23} + 129q^{22} + 145q^{21} + 172q^{20} + 186q^{19} + 210q^{18} + 219q^{17} + 237q^{16} + 238q^{15} \\
 &\quad + 251q^{14} + 238q^{13} + 237q^{12} + 219q^{11} + 210q^{10} + 186q^9 + 172q^8 + 145q^7 + 129q^6 + 102q^5 \\
 &\quad + 87q^4 + 66q^3 + 55q^2 + 38q + 30 + \frac{19}{q} + \frac{14}{q^2} + \frac{8}{q^3} + \frac{6}{q^4} + \frac{2}{q^5} + \frac{2}{q^6} \\
 f_{49}(q) &= -2q^{36} - 2q^{35} - 6q^{34} - 7q^{33} - 10q^{32} - 10q^{31} - 15q^{30} - 10q^{29} - 10q^{28} - 7q^{27} - 6q^{26} - 2q^{25} \\
 &\quad - 2q^{24} \\
 f_{51}(q) &= q^{40} + 5q^{39} + 4q^{38} + 7q^{37} + 13q^{36} + 19q^{35} + 27q^{34} + 39q^{33} + 52q^{32} + 72q^{31} + 93q^{30} + 118q^{29}
 \end{aligned}$$

$$\begin{aligned}
& + 146q^{28} + 182q^{27} + 214q^{26} + 254q^{25} + 296q^{24} + 338q^{23} + 377q^{22} + 419q^{21} + 452q^{20} \\
& + 486q^{19} + 511q^{18} + 531q^{17} + 542q^{16} + 554q^{15} + 542q^{14} + 531q^{13} + 511q^{12} + 486q^{11} \\
& + 452q^{10} + 419q^9 + 377q^8 + 338q^7 + 296q^6 + 254q^5 + 214q^4 + 182q^3 + 146q^2 + 118q \\
& + 93 + \frac{72}{q} + \frac{52}{q^2} + \frac{39}{q^3} + \frac{27}{q^4} + \frac{19}{q^5} + \frac{13}{q^6} + \frac{7}{q^7} + \frac{4}{q^8} + \frac{3}{q^9} + \frac{1}{q^{10}} \\
f_{53}(q) = & -q^{42} - 3q^{41} - 4q^{40} - 7q^{39} - 11q^{38} - 15q^{37} - 18q^{36} - 21q^{35} - 23q^{34} - 27q^{33} - 23q^{32} \\
& - 21q^{31} - 18q^{30} - 15q^{29} - 11q^{28} - 7q^{27} - 4q^{26} - 3q^{25} - q^{24} \\
f_{55}(q) = & 2q^{46} + 3q^{45} + 9q^{44} + 9q^{43} + 14q^{42} + 20q^{41} + 33q^{40} + 42q^{39} + 62q^{38} + 81q^{37} + 110q^{36} \\
& + 137q^{35} + 182q^{34} + 219q^{33} + 277q^{32} + 329q^{31} + 399q^{30} + 460q^{29} + 545q^{28} + 612q^{27} \\
& + 705q^{26} + 778q^{25} + 869q^{24} + 935q^{23} + 1022q^{22} + 1073q^{21} + 1143q^{20} + 1178q^{19} + 1224q^{18} \\
& + 1232q^{17} + 1259q^{16} + 1232q^{15} + 1224q^{14} + 1178q^{13} + 1143q^{12} + 1073q^{11} + 1022q^{10} \\
& + 935q^9 + 869q^8 + 778q^7 + 705q^6 + 612q^5 + 545q^4 + 460q^3 + 399q^2 + 329q + 277 + \frac{219}{q} \\
& + \frac{182}{q^2} + \frac{137}{q^3} + \frac{110}{q^4} + \frac{81}{q^5} + \frac{62}{q^6} + \frac{42}{q^7} + \frac{33}{q^8} + \frac{20}{q^9} + \frac{14}{q^{10}} + \frac{8}{q^{11}} + \frac{6}{q^{12}} + \frac{2}{q^{13}} + \frac{2}{q^{14}} \\
f_{57}(q) = & -2q^{48} - 2q^{47} - 6q^{46} - 8q^{45} - 13q^{44} - 16q^{43} - 26q^{42} - 29q^{41} - 38q^{40} - 41q^{39} - 48q^{38} \\
& - 48q^{37} - 56q^{36} - 48q^{35} - 48q^{34} - 41q^{33} - 38q^{32} - 29q^{31} - 26q^{30} - 16q^{29} - 13q^{28} - 8q^{27} \\
& - 6q^{26} - 2q^{25} - 2q^{24} \\
f_{59}(q) = & q^{53} + 3q^{52} + 6q^{51} + 9q^{50} + 18q^{49} + 21q^{48} + 31q^{47} + 41q^{46} + 58q^{45} + 80q^{44} + 108q^{43} \\
& + 142q^{42} + 186q^{41} + 235q^{40} + 296q^{39} + 367q^{38} + 452q^{37} + 543q^{36} + 652q^{35} + 767q^{34} \\
& + 899q^{33} + 1036q^{32} + 1187q^{31} + 1339q^{30} + 1506q^{29} + 1669q^{28} + 1839q^{27} + 2000q^{26} \\
& + 2162q^{25} + 2307q^{24} + 2449q^{23} + 2567q^{22} + 2676q^{21} + 2756q^{20} + 2822q^{19} + 2856q^{18} \\
& + 2879q^{17} + 2856q^{16} + 2822q^{15} + 2756q^{14} + 2676q^{13} + 2567q^{12} + 2449q^{11} + 2307q^{10} \\
& + 2162q^9 + 2000q^8 + 1839q^7 + 1669q^6 + 1506q^5 + 1339q^4 + 1187q^3 + 1036q^2 + 899q \\
& + 767 + \frac{652}{q} + \frac{543}{q^2} + \frac{452}{q^3} + \frac{367}{q^4} + \frac{296}{q^5} + \frac{235}{q^6} + \frac{186}{q^7} + \frac{142}{q^8} + \frac{108}{q^9} + \frac{80}{q^{10}} + \frac{58}{q^{11}} + \frac{41}{q^{12}} \\
& + \frac{29}{q^{13}} + \frac{19}{q^{14}} + \frac{13}{q^{15}} + \frac{7}{q^{16}} + \frac{4}{q^{17}} + \frac{3}{q^{18}} + \frac{1}{q^{19}} \\
f_{61}(q) = & -q^{55} - 3q^{54} - 4q^{53} - 7q^{52} - 13q^{51} - 17q^{50} - 25q^{49} - 33q^{48} - 43q^{47} - 54q^{46} - 67q^{45} \\
& - 77q^{44} - 88q^{43} - 97q^{42} - 104q^{41} - 108q^{40} - 115q^{39} - 108q^{38} - 104q^{37} - 97q^{36} - 88q^{35} \\
& - 77q^{34} - 67q^{33} - 54q^{32} - 43q^{31} - 33q^{30} - 25q^{29} - 17q^{28} - 13q^{27} - 7q^{26} - 4q^{25} - 3q^{24} \\
& - q^{23} \\
f_{63}(q) = & 2q^{60} + 2q^{59} + 7q^{58} + 11q^{57} + 18q^{56} + 25q^{55} + 42q^{54} + 50q^{53} + 70q^{52} + 91q^{51} + 124q^{50} \\
& + 158q^{49} + 215q^{48} + 268q^{47} + 349q^{46} + 431q^{45} + 541q^{44} + 655q^{43} + 807q^{42} + 954q^{41} \\
& + 1148q^{40} + 1341q^{39} + 1579q^{38} + 1810q^{37} + 2096q^{36} + 2363q^{35} + 2686q^{34} + 2989q^{33} \\
& + 3336q^{32} + 3655q^{31} + 4026q^{30} + 4343q^{29} + 4706q^{28} + 5011q^{27} + 5345q^{26} + 5608q^{25} \\
& + 5901q^{24} + 6103q^{23} + 6327q^{22} + 6459q^{21} + 6599q^{20} + 6641q^{19} + 6702q^{18} + 6641q^{17}
\end{aligned}$$

$$\begin{aligned}
& + 6599q^{16} + 6459q^{15} + 6327q^{14} + 6103q^{13} + 5901q^{12} + 5608q^{11} + 5345q^{10} + 5011q^9 \\
& + 4706q^8 + 4343q^7 + 4026q^6 + 3655q^5 + 3336q^4 + 2989q^3 + 2686q^2 + 2363q + 2096 \\
& + \frac{1810}{q} + \frac{1579}{q^2} + \frac{1341}{q^3} + \frac{1148}{q^4} + \frac{954}{q^5} + \frac{807}{q^6} + \frac{655}{q^7} + \frac{541}{q^8} + \frac{431}{q^9} + \frac{349}{q^{10}} + \frac{268}{q^{11}} + \frac{215}{q^{12}} \\
& + \frac{158}{q^{13}} + \frac{123}{q^{14}} + \frac{88}{q^{15}} + \frac{66}{q^{16}} + \frac{45}{q^{17}} + \frac{34}{q^{18}} + \frac{20}{q^{19}} + \frac{14}{q^{20}} + \frac{8}{q^{21}} + \frac{6}{q^{22}} + \frac{2}{q^{23}} + \frac{2}{q^{24}} \\
f_{65}(q) = & - 3q^{62} - 2q^{61} - 6q^{60} - 8q^{59} - 14q^{58} - 19q^{57} - 30q^{56} - 38q^{55} - 55q^{54} - 66q^{53} - 87q^{52} \\
& - 102q^{51} - 129q^{50} - 145q^{49} - 172q^{48} - 186q^{47} - 210q^{46} - 219q^{45} - 237q^{44} - 238q^{43} \\
& - 251q^{42} - 238q^{41} - 237q^{40} - 219q^{39} - 210q^{38} - 186q^{37} - 172q^{36} - 145q^{35} - 129q^{34} \\
& - 102q^{33} - 87q^{32} - 66q^{31} - 55q^{30} - 38q^{29} - 30q^{28} - 19q^{27} - 14q^{26} - 8q^{25} - 6q^{24} - 2q^{23} \\
& - 2q^{22} \\
f_{67}(q) = & q^{68} + 3q^{67} + 4q^{66} + 9q^{65} + 15q^{64} + 25q^{63} + 36q^{62} + 53q^{61} + 70q^{60} + 101q^{59} + 126q^{58} \\
& + 166q^{57} + 214q^{56} + 279q^{55} + 350q^{54} + 446q^{53} + 560q^{52} + 698q^{51} + 858q^{50} + 1052q^{49} \\
& + 1268q^{48} + 1525q^{47} + 1812q^{46} + 2137q^{45} + 2500q^{44} + 2913q^{43} + 3351q^{42} + 3843q^{41} \\
& + 4369q^{40} + 4940q^{39} + 5536q^{38} + 6182q^{37} + 6838q^{36} + 7536q^{35} + 8239q^{34} + 8962q^{33} \\
& + 9682q^{32} + 10416q^{31} + 11111q^{30} + 11806q^{29} + 12458q^{28} + 13081q^{27} + 13639q^{26} \\
& + 14163q^{25} + 14598q^{24} + 14985q^{23} + 15278q^{22} + 15501q^{21} + 15624q^{20} + 15689q^{19} \\
& + 15624q^{18} + 15501q^{17} + 15278q^{16} + 14985q^{15} + 14598q^{14} + 14163q^{13} + 13639q^{12} \\
& + 13081q^{11} + 12458q^{10} + 11806q^9 + 11111q^8 + 10416q^7 + 9682q^6 + 8962q^5 + 8239q^4 \\
& + 7536q^3 + 6838q^2 + 6182q + 5536 + \frac{4940}{q} + \frac{4369}{q^2} + \frac{3843}{q^3} + \frac{3351}{q^4} + \frac{2913}{q^5} + \frac{2500}{q^6} \\
& + \frac{2137}{q^7} + \frac{1812}{q^8} + \frac{1525}{q^9} + \frac{1268}{q^{10}} + \frac{1052}{q^{11}} + \frac{858}{q^{12}} + \frac{698}{q^{13}} + \frac{560}{q^{14}} + \frac{444}{q^{15}} + \frac{348}{q^{16}} + \frac{273}{q^{17}} \\
& + \frac{207}{q^{18}} + \frac{156}{q^{19}} + \frac{116}{q^{20}} + \frac{86}{q^{21}} + \frac{60}{q^{22}} + \frac{43}{q^{23}} + \frac{29}{q^{24}} + \frac{19}{q^{25}} + \frac{13}{q^{26}} + \frac{7}{q^{27}} + \frac{4}{q^{28}} + \frac{3}{q^{29}} + \frac{1}{q^{30}} \\
f_{69}(q) = & - q^{70} - 5q^{69} - 4q^{68} - 7q^{67} - 13q^{66} - 19q^{65} - 27q^{64} - 39q^{63} - 52q^{62} - 72q^{61} - 93q^{60} \\
& - 118q^{59} - 146q^{58} - 182q^{57} - 214q^{56} - 254q^{55} - 296q^{54} - 338q^{53} - 377q^{52} - 419q^{51} \\
& - 452q^{50} - 486q^{49} - 511q^{48} - 531q^{47} - 542q^{46} - 554q^{45} - 542q^{44} - 531q^{43} - 511q^{42} \\
& - 486q^{41} - 452q^{40} - 419q^{39} - 377q^{38} - 338q^{37} - 296q^{36} - 254q^{35} - 214q^{34} - 182q^{33} \\
& - 146q^{32} - 118q^{31} - 93q^{30} - 72q^{29} - 52q^{28} - 39q^{27} - 27q^{26} - 19q^{25} - 13q^{24} - 7q^{23} \\
& - 4q^{22} - 3q^{21} - q^{20} \\
f_{71}(q) = & 2q^{76} + 2q^{75} + 6q^{74} + 9q^{73} + 17q^{72} + 24q^{71} + 41q^{70} + 57q^{69} + 84q^{68} + 110q^{67} + 151q^{66} \\
& + 194q^{65} + 261q^{64} + 322q^{63} + 417q^{62} + 517q^{61} + 656q^{60} + 804q^{59} + 1004q^{58} + 1219q^{57} \\
& + 1503q^{56} + 1802q^{55} + 2180q^{54} + 2585q^{53} + 3082q^{52} + 3605q^{51} + 4238q^{50} + 4897q^{49} \\
& + 5676q^{48} + 6485q^{47} + 7425q^{46} + 8387q^{45} + 9491q^{44} + 10605q^{43} + 11861q^{42} + 13119q^{41} \\
& + 14514q^{40} + 15887q^{39} + 17393q^{38} + 18850q^{37} + 20424q^{36} + 21923q^{35} + 23519q^{34} \\
& + 25002q^{33} + 26562q^{32} + 27969q^{31} + 29425q^{30} + 30697q^{29} + 31988q^{28} + 33059q^{27}
\end{aligned}$$

$$\begin{aligned}
& + 34130q^{26} + 34947q^{25} + 35742q^{24} + 36264q^{23} + 36746q^{22} + 36941q^{21} + 37095q^{20} \\
& + 36941q^{19} + 36746q^{18} + 36264q^{17} + 35742q^{16} + 34947q^{15} + 34130q^{14} + 33059q^{13} \\
& + 31988q^{12} + 30697q^{11} + 29425q^{10} + 27969q^9 + 26562q^8 + 25002q^7 + 23519q^6 + 21923q^5 \\
& + 20424q^4 + 18850q^3 + 17393q^2 + 15887q + 14514 + \frac{13119}{q} + \frac{11861}{q^2} + \frac{10605}{q^3} + \frac{9491}{q^4} \\
& + \frac{8387}{q^5} + \frac{7425}{q^6} + \frac{6485}{q^7} + \frac{5676}{q^8} + \frac{4897}{q^9} + \frac{4238}{q^{10}} + \frac{3605}{q^{11}} + \frac{3082}{q^{12}} + \frac{2585}{q^{13}} + \frac{2180}{q^{14}} + \frac{1801}{q^{15}} \\
& + \frac{1500}{q^{16}} + \frac{1215}{q^{17}} + \frac{997}{q^{18}} + \frac{793}{q^{19}} + \frac{641}{q^{20}} + \frac{499}{q^{21}} + \frac{396}{q^{22}} + \frac{299}{q^{23}} + \frac{234}{q^{24}} + \frac{171}{q^{25}} + \frac{130}{q^{26}} + \frac{92}{q^{27}} \\
& + \frac{69}{q^{28}} + \frac{46}{q^{29}} + \frac{34}{q^{30}} + \frac{20}{q^{31}} + \frac{14}{q^{32}} + \frac{8}{q^{33}} + \frac{6}{q^{34}} + \frac{2}{q^{35}} + \frac{2}{q^{36}} \\
f_{73}(q) = & - 2q^{78} - 3q^{77} - 9q^{76} - 9q^{75} - 14q^{74} - 20q^{73} - 33q^{72} - 42q^{71} - 62q^{70} - 81q^{69} - 110q^{68} \\
& - 137q^{67} - 182q^{66} - 219q^{65} - 277q^{64} - 329q^{63} - 399q^{62} - 460q^{61} - 545q^{60} - 612q^{59} \\
& - 705q^{58} - 778q^{57} - 869q^{56} - 935q^{55} - 1022q^{54} - 1073q^{53} - 1143q^{52} - 1178q^{51} - 1224q^{50} \\
& - 1232q^{49} - 1259q^{48} - 1232q^{47} - 1224q^{46} - 1178q^{45} - 1143q^{44} - 1073q^{43} - 1022q^{42} \\
& - 935q^{41} - 869q^{40} - 778q^{39} - 705q^{38} - 612q^{37} - 545q^{36} - 460q^{35} - 399q^{34} - 329q^{33} \\
& - 277q^{32} - 219q^{31} - 182q^{30} - 137q^{29} - 110q^{28} - 81q^{27} - 62q^{26} - 42q^{25} - 33q^{24} - 20q^{23} \\
& - 14q^{22} - 8q^{21} - 6q^{20} - 2q^{19} - 2q^{18} \\
f_{75}(q) = & q^{85} + 3q^{84} + 4q^{83} + 7q^{82} + 15q^{81} + 21q^{80} + 35q^{79} + 51q^{78} + 75q^{77} + 104q^{76} + 148q^{75} \\
& + 193q^{74} + 259q^{73} + 334q^{72} + 431q^{71} + 542q^{70} + 692q^{69} + 849q^{68} + 1056q^{67} + 1296q^{66} \\
& + 1588q^{65} + 1925q^{64} + 2337q^{63} + 2800q^{62} + 3358q^{61} + 3992q^{60} + 4725q^{59} + 5553q^{58} \\
& + 6509q^{57} + 7563q^{56} + 8759q^{55} + 10081q^{54} + 11549q^{53} + 13152q^{52} + 14925q^{51} + 16826q^{50} \\
& + 18908q^{49} + 21128q^{48} + 23514q^{47} + 26035q^{46} + 28729q^{45} + 31522q^{44} + 34474q^{43} \\
& + 37517q^{42} + 40677q^{41} + 43891q^{40} + 47204q^{39} + 50512q^{38} + 53878q^{37} + 57207q^{36} \\
& + 60521q^{35} + 63744q^{34} + 66919q^{33} + 69921q^{32} + 72821q^{31} + 75512q^{30} + 78028q^{29} \\
& + 80280q^{28} + 82330q^{27} + 84052q^{26} + 85533q^{25} + 86669q^{24} + 87516q^{23} + 87998q^{22} \\
& + 88202q^{21} + 87998q^{20} + 87516q^{19} + 86669q^{18} + 85533q^{17} + 84052q^{16} + 82330q^{15} \\
& + 80280q^{14} + 78028q^{13} + 75512q^{12} + 72821q^{11} + 69921q^{10} + 66919q^9 + 63744q^8 \\
& + 60521q^7 + 57207q^6 + 53878q^5 + 50512q^4 + 47204q^3 + 43891q^2 + 40677q + 37517 \\
& + \frac{34474}{q} + \frac{31522}{q^2} + \frac{28729}{q^3} + \frac{26035}{q^4} + \frac{23514}{q^5} + \frac{21128}{q^6} + \frac{18908}{q^7} + \frac{16826}{q^8} + \frac{14925}{q^9} \\
& + \frac{13152}{q^{10}} + \frac{11549}{q^{11}} + \frac{10081}{q^{12}} + \frac{8759}{q^{13}} + \frac{7563}{q^{14}} + \frac{6507}{q^{15}} + \frac{5551}{q^{16}} + \frac{4719}{q^{17}} + \frac{3984}{q^{18}} + \frac{3345}{q^{19}} \\
& + \frac{2784}{q^{20}} + \frac{2311}{q^{21}} + \frac{1896}{q^{22}} + \frac{1550}{q^{23}} + \frac{1255}{q^{24}} + \frac{1008}{q^{25}} + \frac{801}{q^{26}} + \frac{636}{q^{27}} + \frac{494}{q^{28}} + \frac{383}{q^{29}} + \frac{293}{q^{30}} \\
& + \frac{221}{q^{31}} + \frac{164}{q^{32}} + \frac{122}{q^{33}} + \frac{88}{q^{34}} + \frac{62}{q^{35}} + \frac{43}{q^{36}} + \frac{29}{q^{37}} + \frac{19}{q^{38}} + \frac{13}{q^{39}} + \frac{7}{q^{40}} + \frac{4}{q^{41}} + \frac{3}{q^{42}} + \frac{1}{q^{43}} \\
f_{77}(q) = & - q^{87} - 3q^{86} - 6q^{85} - 9q^{84} - 18q^{83} - 21q^{82} - 31q^{81} - 41q^{80} - 58q^{79} - 80q^{78} - 108q^{77}
\end{aligned}$$

$$\begin{aligned}
& -142q^{76} - 186q^{75} - 235q^{74} - 296q^{73} - 367q^{72} - 452q^{71} - 543q^{70} - 652q^{69} - 767q^{68} \\
& - 899q^{67} - 1036q^{66} - 1187q^{65} - 1339q^{64} - 1506q^{63} - 1669q^{62} - 1839q^{61} - 2000q^{60} \\
& - 2162q^{59} - 2307q^{58} - 2449q^{57} - 2567q^{56} - 2676q^{55} - 2756q^{54} - 2822q^{53} - 2856q^{52} \\
& - 2879q^{51} - 2856q^{50} - 2822q^{49} - 2756q^{48} - 2676q^{47} - 2567q^{46} - 2449q^{45} - 2307q^{44} \\
& - 2162q^{43} - 2000q^{42} - 1839q^{41} - 1669q^{40} - 1506q^{39} - 1339q^{38} - 1187q^{37} - 1036q^{36} \\
& - 899q^{35} - 767q^{34} - 652q^{33} - 543q^{32} - 452q^{31} - 367q^{30} - 296q^{29} - 235q^{28} - 186q^{27} \\
& - 142q^{26} - 108q^{25} - 80q^{24} - 58q^{23} - 41q^{22} - 29q^{21} - 19q^{20} - 13q^{19} - 7q^{18} - 4q^{17} - 3q^{16} \\
& - q^{15} \\
f_{79}(q) = & 2q^{94} + 2q^{93} + 6q^{92} + 8q^{91} + 15q^{90} + 23q^{89} + 38q^{88} + 53q^{87} + 83q^{86} + 112q^{85} + 159q^{84} \\
& + 211q^{83} + 290q^{82} + 372q^{81} + 492q^{80} + 621q^{79} + 795q^{78} + 986q^{77} + 1237q^{76} + 1509q^{75} \\
& + 1870q^{74} + 2256q^{73} + 2747q^{72} + 3291q^{71} + 3968q^{70} + 4708q^{69} + 5618q^{68} + 6618q^{67} \\
& + 7815q^{66} + 9126q^{65} + 10683q^{64} + 12365q^{63} + 14337q^{62} + 16460q^{61} + 18898q^{60} \\
& + 21518q^{59} + 24498q^{58} + 27655q^{57} + 31208q^{56} + 34961q^{55} + 39122q^{54} + 43481q^{53} \\
& + 48283q^{52} + 53251q^{51} + 58671q^{50} + 64247q^{49} + 70248q^{48} + 76369q^{47} + 82909q^{46} \\
& + 89489q^{45} + 96453q^{44} + 103408q^{43} + 110671q^{42} + 117835q^{41} + 125260q^{40} \\
& + 132470q^{39} + 139865q^{38} + 146953q^{37} + 154109q^{36} + 160849q^{35} + 167589q^{34} \\
& + 173771q^{33} + 179860q^{32} + 185309q^{31} + 190550q^{30} + 195053q^{29} + 199295q^{28} \\
& + 202693q^{27} + 205766q^{26} + 207955q^{25} + 209750q^{24} + 210625q^{23} + 211113q^{22} \\
& + 210625q^{21} + 209750q^{20} + 207955q^{19} + 205766q^{18} + 202693q^{17} + 199295q^{16} \\
& + 195053q^{15} + 190550q^{14} + 185309q^{13} + 179860q^{12} + 173771q^{11} + 167589q^{10} \\
& + 160849q^9 + 154109q^8 + 146953q^7 + 139865q^6 + 132470q^5 + 125260q^4 + 117835q^3 \\
& + 110671q^2 + 103408q + 96453 + \frac{89489}{q} + \frac{82909}{q^2} + \frac{76369}{q^3} + \frac{70248}{q^4} + \frac{64247}{q^5} + \frac{58671}{q^6} \\
& + \frac{53251}{q^7} + \frac{48283}{q^8} + \frac{43481}{q^9} + \frac{39122}{q^{10}} + \frac{34961}{q^{11}} + \frac{31208}{q^{12}} + \frac{27655}{q^{13}} + \frac{24497}{q^{14}} + \frac{21515}{q^{15}} \\
& + \frac{18894}{q^{16}} + \frac{16453}{q^{17}} + \frac{14324}{q^{18}} + \frac{12348}{q^{19}} + \frac{10658}{q^{20}} + \frac{9093}{q^{21}} + \frac{7772}{q^{22}} + \frac{6564}{q^{23}} + \frac{5551}{q^{24}} + \frac{4631}{q^{25}} \\
& + \frac{3880}{q^{26}} + \frac{3194}{q^{27}} + \frac{2643}{q^{28}} + \frac{2148}{q^{29}} + \frac{1755}{q^{30}} + \frac{1401}{q^{31}} + \frac{1133}{q^{32}} + \frac{889}{q^{33}} + \frac{707}{q^{34}} + \frac{544}{q^{35}} + \frac{425}{q^{36}} + \frac{318}{q^{37}} \\
& + \frac{247}{q^{38}} + \frac{178}{q^{39}} + \frac{134}{q^{40}} + \frac{95}{q^{41}} + \frac{70}{q^{42}} + \frac{46}{q^{43}} + \frac{34}{q^{44}} + \frac{20}{q^{45}} + \frac{14}{q^{46}} + \frac{8}{q^{47}} + \frac{6}{q^{48}} + \frac{2}{q^{49}} + \frac{2}{q^{50}} \\
f_{81}(q) = & -2q^{96} - 2q^{95} - 7q^{94} - 11q^{93} - 18q^{92} - 25q^{91} - 42q^{90} - 50q^{89} - 70q^{88} - 91q^{87} - 124q^{86} \\
& - 158q^{85} - 215q^{84} - 268q^{83} - 349q^{82} - 431q^{81} - 541q^{80} - 655q^{79} - 807q^{78} - 954q^{77} \\
& - 1148q^{76} - 1341q^{75} - 1579q^{74} - 1810q^{73} - 2096q^{72} - 2363q^{71} - 2686q^{70} - 2989q^{69} \\
& - 3336q^{68} - 3655q^{67} - 4026q^{66} - 4343q^{65} - 4706q^{64} - 5011q^{63} - 5345q^{62} - 5608q^{61} \\
& - 5901q^{60} - 6103q^{59} - 6327q^{58} - 6459q^{57} - 6599q^{56} - 6641q^{55} - 6702q^{54} - 6641q^{53} \\
& - 6599q^{52} - 6459q^{51} - 6327q^{50} - 6103q^{49} - 5901q^{48} - 5608q^{47} - 5345q^{46} - 5011q^{45}
\end{aligned}$$

$$\begin{aligned}
& -4706q^{44} - 4343q^{43} - 4026q^{42} - 3655q^{41} - 3336q^{40} - 2989q^{39} - 2686q^{38} - 2363q^{37} \\
& - 2096q^{36} - 1810q^{35} - 1579q^{34} - 1341q^{33} - 1148q^{32} - 954q^{31} - 807q^{30} - 655q^{29} - 541q^{28} \\
& - 431q^{27} - 349q^{26} - 268q^{25} - 215q^{24} - 158q^{23} - 123q^{22} - 88q^{21} - 66q^{20} - 45q^{19} - 34q^{18} \\
& - 20q^{17} - 14q^{16} - 8q^{15} - 6q^{14} - 2q^{13} - 2q^{12} \\
f_{83}(q) = & q^{104} + 3q^{103} + 4q^{102} + 7q^{101} + 13q^{100} + 22q^{99} + 31q^{98} + 49q^{97} + 70q^{96} + 104q^{95} \\
& + 143q^{94} + 200q^{93} + 267q^{92} + 362q^{91} + 469q^{90} + 615q^{89} + 785q^{88} + 1004q^{87} + 1255q^{86} \\
& + 1572q^{85} + 1934q^{84} + 2385q^{83} + 2896q^{82} + 3518q^{81} + 4232q^{80} + 5092q^{79} + 6058q^{78} \\
& + 7209q^{77} + 8518q^{76} + 10050q^{75} + 11783q^{74} + 13792q^{73} + 16049q^{72} + 18640q^{71} \\
& + 21530q^{70} + 24809q^{69} + 28458q^{68} + 32550q^{67} + 37056q^{66} + 42074q^{65} + 47562q^{64} \\
& + 53611q^{63} + 60179q^{62} + 67353q^{61} + 75086q^{60} + 83471q^{59} + 92432q^{58} + 102059q^{57} \\
& + 112288q^{56} + 123190q^{55} + 134666q^{54} + 146812q^{53} + 159497q^{52} + 172808q^{51} \\
& + 186601q^{50} + 200949q^{49} + 215696q^{48} + 230912q^{47} + 246398q^{46} + 262233q^{45} \\
& + 278215q^{44} + 294397q^{43} + 310547q^{42} + 326745q^{41} + 342737q^{40} + 358588q^{39} \\
& + 374042q^{38} + 389156q^{37} + 403679q^{36} + 417684q^{35} + 430885q^{34} + 443382q^{33} \\
& + 454907q^{32} + 465550q^{31} + 475049q^{30} + 483527q^{29} + 490725q^{28} + 496781q^{27} \\
& + 501455q^{26} + 504899q^{25} + 506903q^{24} + 507651q^{23} + 506903q^{22} + 504899q^{21} \\
& + 501455q^{20} + 496781q^{19} + 490725q^{18} + 483527q^{17} + 475049q^{16} + 465550q^{15} \\
& + 454907q^{14} + 443382q^{13} + 430885q^{12} + 417684q^{11} + 403679q^{10} + 389156q^9 \\
& + 374042q^8 + 358588q^7 + 342737q^6 + 326745q^5 + 310547q^4 + 294397q^3 + 278215q^2 \\
& + 262233q + 246398 + \frac{230912}{q} + \frac{215696}{q^2} + \frac{200949}{q^3} + \frac{186601}{q^4} + \frac{172808}{q^5} + \frac{159497}{q^6} \\
& + \frac{146812}{q^7} + \frac{134666}{q^8} + \frac{123190}{q^9} + \frac{112288}{q^{10}} + \frac{102059}{q^{11}} + \frac{92432}{q^{12}} + \frac{83469}{q^{13}} + \frac{75084}{q^{14}} \\
& + \frac{67347}{q^{15}} + \frac{60171}{q^{16}} + \frac{53597}{q^{17}} + \frac{47543}{q^{18}} + \frac{42044}{q^{19}} + \frac{37018}{q^{20}} + \frac{32495}{q^{21}} + \frac{28392}{q^{22}} \\
& + \frac{24722}{q^{23}} + \frac{21428}{q^{24}} + \frac{18511}{q^{25}} + \frac{15904}{q^{26}} + \frac{13620}{q^{27}} + \frac{11597}{q^{28}} + \frac{9840}{q^{29}} + \frac{8299}{q^{30}} + \frac{6972}{q^{31}} \\
& + \frac{5820}{q^{32}} + \frac{4841}{q^{33}} + \frac{3994}{q^{34}} + \frac{3281}{q^{35}} + \frac{2677}{q^{36}} + \frac{2175}{q^{37}} + \frac{1748}{q^{38}} + \frac{1400}{q^{39}} + \frac{1110}{q^{40}} + \frac{875}{q^{41}} \\
& + \frac{683}{q^{42}} + \frac{528}{q^{43}} + \frac{403}{q^{44}} + \frac{307}{q^{45}} + \frac{229}{q^{46}} + \frac{170}{q^{47}} + \frac{124}{q^{48}} + \frac{90}{q^{49}} + \frac{62}{q^{50}} + \frac{43}{q^{51}} + \frac{29}{q^{52}} + \frac{19}{q^{53}} + \frac{13}{q^{54}} \\
& + \frac{7}{q^{55}} + \frac{4}{q^{56}} + \frac{3}{q^{57}} + \frac{1}{q^{58}} \\
f_{85}(q) = & -q^{106} - 3q^{105} - 4q^{104} - 9q^{103} - 15q^{102} - 25q^{101} - 36q^{100} - 53q^{99} - 70q^{98} - 101q^{97} \\
& - 126q^{96} - 166q^{95} - 214q^{94} - 279q^{93} - 350q^{92} - 446q^{91} - 560q^{90} - 698q^{89} - 858q^{88} \\
& - 1052q^{87} - 1268q^{86} - 1525q^{85} - 1812q^{84} - 2137q^{83} - 2500q^{82} - 2913q^{81} - 3351q^{80} \\
& - 3843q^{79} - 4369q^{78} - 4940q^{77} - 5536q^{76} - 6182q^{75} - 6838q^{74} - 7536q^{73} - 8239q^{72} \\
& - 8962q^{71} - 9682q^{70} - 10416q^{69} - 11111q^{68} - 11806q^{67} - 12458q^{66} - 13081q^{65}
\end{aligned}$$

$$\begin{aligned}
& -13639q^{64} - 14163q^{63} - 14598q^{62} - 14985q^{61} - 15278q^{60} - 15501q^{59} - 15624q^{58} \\
& - 15689q^{57} - 15624q^{56} - 15501q^{55} - 15278q^{54} - 14985q^{53} - 14598q^{52} - 14163q^{51} \\
& - 13639q^{50} - 13081q^{49} - 12458q^{48} - 11806q^{47} - 11111q^{46} - 10416q^{45} - 9682q^{44} \\
& - 8962q^{43} - 8239q^{42} - 7536q^{41} - 6838q^{40} - 6182q^{39} - 5536q^{38} - 4940q^{37} - 4369q^{36} \\
& - 3843q^{35} - 3351q^{34} - 2913q^{33} - 2500q^{32} - 2137q^{31} - 1812q^{30} - 1525q^{29} - 1268q^{28} \\
& - 1052q^{27} - 858q^{26} - 698q^{25} - 560q^{24} - 444q^{23} - 348q^{22} - 273q^{21} - 207q^{20} - 156q^{19} \\
& - 116q^{18} - 86q^{17} - 60q^{16} - 43q^{15} - 29q^{14} - 19q^{13} - 13q^{12} - 7q^{11} - 4q^{10} - 3q^9 - q^8 \\
f_{87}(q) = & 2q^{114} + 2q^{113} + 6q^{112} + 8q^{111} + 14q^{110} + 21q^{109} + 39q^{108} + 50q^{107} + 77q^{106} + 109q^{105} \\
& + 156q^{104} + 209q^{103} + 293q^{102} + 383q^{101} + 516q^{100} + 666q^{99} + 868q^{98} + 1099q^{97} + 1409q^{96} \\
& + 1747q^{95} + 2193q^{94} + 2695q^{93} + 3322q^{92} + 4028q^{91} + 4907q^{90} + 5882q^{89} + 7077q^{88} \\
& + 8415q^{87} + 10018q^{86} + 11812q^{85} + 13959q^{84} + 16323q^{83} + 19124q^{82} + 22236q^{81} \\
& + 25858q^{80} + 29865q^{79} + 34504q^{78} + 39597q^{77} + 45439q^{76} + 51840q^{75} + 59094q^{74} \\
& + 67006q^{73} + 75920q^{72} + 85556q^{71} + 96322q^{70} + 107928q^{69} + 120758q^{68} \\
& + 134506q^{67} + 149618q^{66} + 165686q^{65} + 183217q^{64} + 201771q^{63} + 221834q^{62} \\
& + 242944q^{61} + 265638q^{60} + 289332q^{59} + 314626q^{58} + 340899q^{57} + 368717q^{56} \\
& + 397416q^{55} + 427625q^{54} + 458540q^{53} + 490853q^{52} + 523715q^{51} + 557774q^{50} \\
& + 592154q^{49} + 627553q^{48} + 662951q^{47} + 699119q^{46} + 735003q^{45} + 771326q^{44} \\
& + 807011q^{43} + 842855q^{42} + 877642q^{41} + 912241q^{40} + 945436q^{39} + 978047q^{38} \\
& + 1008868q^{37} + 1038799q^{36} + 1066518q^{35} + 1093018q^{34} + 1117004q^{33} + 1139426q^{32} \\
& + 1159030q^{31} + 1176852q^{30} + 1191564q^{29} + 1204290q^{28} + 1213761q^{27} + 1221060q^{26} \\
& + 1224988q^{25} + 1226724q^{24} + 1224988q^{23} + 1221060q^{22} + 1213761q^{21} + 1204290q^{20} \\
& + 1191564q^{19} + 1176852q^{18} + 1159030q^{17} + 1139426q^{16} + 1117004q^{15} + 1093018q^{14} \\
& + 1066518q^{13} + 1038799q^{12} + 1008868q^{11} + 978047q^{10} + 945436q^9 + 912241q^8 + 877642q^7 \\
& + 842855q^6 + 807011q^5 + 771326q^4 + 735003q^3 + 699119q^2 + 662951q + 627553 + \frac{592154}{q} \\
& + \frac{557774}{q^2} + \frac{523715}{q^3} + \frac{490853}{q^4} + \frac{458540}{q^5} + \frac{427625}{q^6} + \frac{397416}{q^7} + \frac{368717}{q^8} + \frac{340899}{q^9} \\
& + \frac{314626}{q^{10}} + \frac{289331}{q^{11}} + \frac{265635}{q^{12}} + \frac{42940}{q^{13}} + \frac{221827}{q^{14}} + \frac{201758}{q^{15}} + \frac{183198}{q^{16}} + \frac{165659}{q^{17}} \\
& + \frac{149579}{q^{18}} + \frac{134454}{q^{19}} + \frac{120686}{q^{20}} + \frac{107835}{q^{21}} + \frac{96204}{q^{22}} + \frac{85410}{q^{23}} + \frac{75738}{q^{24}} + \frac{66792}{q^{25}} + \frac{58840}{q^{26}} \\
& + \frac{51544}{q^{27}} + \frac{45101}{q^{28}} + \frac{39220}{q^{29}} + \frac{34085}{q^{30}} + \frac{29413}{q^{31}} + \frac{25372}{q^{32}} + \frac{21725}{q^{33}} + \frac{18593}{q^{34}} + \frac{15781}{q^{35}} \\
& + \frac{13405}{q^{36}} + \frac{11270}{q^{37}} + \frac{9487}{q^{38}} + \frac{7904}{q^{39}} + \frac{6591}{q^{40}} + \frac{5430}{q^{41}} + \frac{4488}{q^{42}} + \frac{3651}{q^{43}} + \frac{2984}{q^{44}} + \frac{2399}{q^{45}} \\
& + \frac{1939}{q^{46}} + \frac{1533}{q^{47}} + \frac{1227}{q^{48}} + \frac{953}{q^{49}} + \frac{750}{q^{50}} + \frac{573}{q^{51}} + \frac{444}{q^{52}} + \frac{331}{q^{53}} + \frac{254}{q^{54}} + \frac{182}{q^{55}} + \frac{137}{q^{56}} + \frac{96}{q^{57}}
\end{aligned}$$

$$\begin{aligned}
& + \frac{70}{q^{58}} + \frac{46}{q^{59}} + \frac{34}{q^{60}} + \frac{20}{q^{61}} + \frac{14}{q^{62}} + \frac{8}{q^{63}} + \frac{6}{q^{64}} + \frac{2}{q^{65}} + \frac{2}{q^{66}} \\
f_{89}(q) = & -2q^{116} - 2q^{115} - 6q^{114} - 9q^{113} - 17q^{112} - 24q^{111} - 41q^{110} - 57q^{109} - 84q^{108} \\
& - 110q^{107} - 151q^{106} - 194q^{105} - 261q^{104} - 322q^{103} - 417q^{102} - 517q^{101} - 656q^{100} \\
& - 804q^{99} - 1004q^{98} - 1219q^{97} - 1503q^{96} - 1802q^{95} - 2180q^{94} - 2585q^{93} - 3082q^{92} \\
& - 3605q^{91} - 4238q^{90} - 4897q^{89} - 5676q^{88} - 6485q^{87} - 7425q^{86} - 8387q^{85} - 9491q^{84} \\
& - 10605q^{83} - 11861q^{82} - 13119q^{81} - 14514q^{80} - 15887q^{79} - 17393q^{78} - 18850q^{77} \\
& - 20424q^{76} - 21923q^{75} - 23519q^{74} - 25002q^{73} - 26562q^{72} - 27969q^{71} - 29425q^{70} \\
& - 30697q^{69} - 31988q^{68} - 33059q^{67} - 34130q^{66} - 34947q^{65} - 35742q^{64} - 36264q^{63} \\
& - 36746q^{62} - 36941q^{61} - 37095q^{60} - 36941q^{59} - 36746q^{58} - 36264q^{57} - 35742q^{56} \\
& - 34947q^{55} - 34130q^{54} - 33059q^{53} - 31988q^{52} - 30697q^{51} - 29425q^{50} - 27969q^{49} \\
& - 26562q^{48} - 25002q^{47} - 23519q^{46} - 21923q^{45} - 20424q^{44} - 18850q^{43} - 17393q^{42} \\
& - 15887q^{41} - 14514q^{40} - 13119q^{39} - 11861q^{38} - 10605q^{37} - 9491q^{36} - 8387q^{35} \\
& - 7425q^{34} - 6485q^{33} - 5676q^{32} - 4897q^{31} - 4238q^{30} - 3605q^{29} - 3082q^{28} - 2585q^{27} \\
& - 2180q^{26} - 1801q^{25} - 1500q^{24} - 1215q^{23} - 997q^{22} - 793q^{21} - 641q^{20} - 499q^{19} - 396q^{18} \\
& - 299q^{17} - 234q^{16} - 171q^{15} - 130q^{14} - 92q^{13} - 69q^{12} - 46q^{11} - 34q^{10} - 20q^9 - 14q^8 - 8q^7 \\
& - 6q^6 - 2q^5 - 2q^4 \\
f_{91}(q) = & q^{125} + 3q^{124} + 4q^{123} + 7q^{122} + 13q^{121} + 19q^{120} + 31q^{119} + 46q^{118} + 71q^{117} + 99q^{116} \\
& + 140q^{115} + 192q^{114} + 268q^{113} + 357q^{112} + 479q^{111} + 629q^{110} + 827q^{109} + 1058q^{108} \\
& + 1363q^{107} + 1719q^{106} + 2169q^{105} + 2697q^{104} + 3350q^{103} + 4104q^{102} + 5031q^{101} \\
& + 6098q^{100} + 7380q^{99} + 8855q^{98} + 10609q^{97} + 12604q^{96} + 14959q^{95} + 17634q^{94} \\
& + 20749q^{93} + 24285q^{92} + 28371q^{91} + 32975q^{90} + 38270q^{89} + 44207q^{88} + 50966q^{87} \\
& + 58539q^{86} + 67106q^{85} + 76634q^{84} + 87349q^{83} + 99224q^{82} + 112469q^{81} \\
& + 127078q^{80} + 143276q^{79} + 161026q^{78} + 180595q^{77} + 201941q^{76} + 225292q^{75} \\
& + 250636q^{74} + 278211q^{73} + 307938q^{72} + 340096q^{71} + 374601q^{70} + 411670q^{69} \\
& + 451230q^{68} + 493505q^{67} + 538336q^{66} + 585975q^{65} + 636236q^{64} + 689293q^{63} \\
& + 744968q^{62} + 803437q^{61} + 864387q^{60} + 928022q^{59} + 994012q^{58} + 1062457q^{57} \\
& + 1133007q^{56} + 1205771q^{55} + 1280263q^{54} + 1356612q^{53} + 1434305q^{52} + 1513364q^{51} \\
& + 1593272q^{50} + 1674065q^{49} + 1755076q^{48} + 1836383q^{47} + 1917323q^{46} + 1997860q^{45} \\
& + 2077343q^{44} + 2155778q^{43} + 2232395q^{42} + 2307259q^{41} + 2379622q^{40} + 2449467q^{39} \\
& + 2516105q^{38} + 2579591q^{37} + 2639132q^{36} + 2694879q^{35} + 2746118q^{34} + 2792934q^{33} \\
& + 2834697q^{32} + 2871604q^{31} + 2902963q^{30} + 2929084q^{29} + 2949378q^{28} + 2964116q^{27} \\
& + 2972831q^{26} + 2975915q^{25} + 2972831q^{24} + 2964116q^{23} + 2949378q^{22} + 2929084q^{21} \\
& + 2902963q^{20} + 2871604q^{19} + 2834697q^{18} + 2792934q^{17} + 2746118q^{16} + 2694879q^{15} \\
& + 2639132q^{14} + 2579591q^{13} + 2516105q^{12} + 2449467q^{11} + 2379622q^{10} + 2307259q^9
\end{aligned}$$



$$\begin{aligned}
& + 2232395q^8 + 2155778q^7 + 2077343q^6 + 1997860q^5 + 1917323q^4 + 1836383q^3 \\
& + 1755076q^2 + 1674065q + 1593272 + \frac{1513364}{q} + \frac{1434305}{q^2} + \frac{1356612}{q^3} + \frac{1280263}{q^4} \\
& + \frac{1205771}{q^5} + \frac{1133007}{q^6} + \frac{1062457}{q^7} + \frac{994012}{q^8} + \frac{928020}{q^9} + \frac{864385}{q^{10}} + \frac{803431}{q^{11}} + \frac{744960}{q^{12}} \\
& + \frac{689279}{q^{13}} + \frac{636216}{q^{14}} + \frac{585942}{q^{15}} + \frac{538294}{q^{16}} + \frac{493443}{q^{17}} + \frac{451149}{q^{18}} + \frac{411560}{q^{19}} + \frac{374464}{q^{20}} \\
& + \frac{339914}{q^{21}} + \frac{307719}{q^{22}} + \frac{277934}{q^{23}} + \frac{250307}{q^{24}} + \frac{224893}{q^{25}} + \frac{201481}{q^{26}} + \frac{180050}{q^{27}} + \frac{160414}{q^{28}} \\
& + \frac{142571}{q^{29}} + \frac{126300}{q^{30}} + \frac{111600}{q^{31}} + \frac{98289}{q^{32}} + \frac{86327}{q^{33}} + \frac{75561}{q^{34}} + \frac{65963}{q^{35}} + \frac{57361}{q^{36}} + \frac{49742}{q^{37}} \\
& + \frac{42975}{q^{38}} + \frac{37011}{q^{39}} + \frac{31743}{q^{40}} + \frac{27147}{q^{41}} + \frac{23107}{q^{42}} + \frac{19606}{q^{43}} + \frac{16561}{q^{44}} + \frac{13937}{q^{45}} + \frac{11669}{q^{46}} \\
& + \frac{9740}{q^{47}} + \frac{8077}{q^{48}} + \frac{6675}{q^{49}} + \frac{5486}{q^{50}} + \frac{4486}{q^{51}} + \frac{3644}{q^{52}} + \frac{2951}{q^{53}} + \frac{2368}{q^{54}} + \frac{1892}{q^{55}} + \frac{1500}{q^{56}} + \frac{1181}{q^{57}} \\
& + \frac{921}{q^{58}} + \frac{717}{q^{59}} + \frac{548}{q^{60}} + \frac{417}{q^{61}} + \frac{315}{q^{62}} + \frac{235}{q^{63}} + \frac{172}{q^{64}} + \frac{126}{q^{65}} + \frac{90}{q^{66}} + \frac{62}{q^{67}} + \frac{43}{q^{68}} + \frac{29}{q^{69}} + \frac{19}{q^{70}} \\
& + \frac{13}{q^{71}} + \frac{7}{q^{72}} + \frac{4}{q^{73}} + \frac{3}{q^{74}} + \frac{1}{q^{75}} \\
f_{93}(q) = & -q^{127} - 3q^{126} - 4q^{125} - 7q^{124} - 15q^{123} - 21q^{122} - 35q^{121} - 51q^{120} - 75q^{119} - 104q^{118} \\
& - 148q^{117} - 193q^{116} - 259q^{115} - 334q^{114} - 431q^{113} - 542q^{112} - 692q^{111} - 849q^{110} \\
& - 1056q^{109} - 1296q^{108} - 1588q^{107} - 1925q^{106} - 2337q^{105} - 2800q^{104} - 3358q^{103} - 3992q^{102} \\
& - 4725q^{101} - 5553q^{100} - 6509q^{99} - 7563q^{98} - 8759q^{97} - 10081q^{96} - 11549q^{95} - 13152q^{94} \\
& - 14925q^{93} - 16826q^{92} - 18908q^{91} - 21128q^{90} - 23514q^{89} - 26035q^{88} - 28729q^{87} \\
& - 31522q^{86} - 34474q^{85} - 37517q^{84} - 40677q^{83} - 43891q^{82} - 47204q^{81} - 50512q^{80} \\
& - 53878q^{79} - 57207q^{78} - 60521q^{77} - 63744q^{76} - 66919q^{75} - 69921q^{74} - 72821q^{73} \\
& - 75512q^{72} - 78028q^{71} - 80280q^{70} - 82330q^{69} - 84052q^{68} - 85533q^{67} - 86669q^{66} \\
& - 87516q^{65} - 87998q^{64} - 88202q^{63} - 87998q^{62} - 87516q^{61} - 86669q^{60} - 85533q^{59} \\
& - 84052q^{58} - 82330q^{57} - 80280q^{56} - 78028q^{55} - 75512q^{54} - 72821q^{53} - 69921q^{52} \\
& - 66919q^{51} - 63744q^{50} - 60521q^{49} - 57207q^{48} - 53878q^{47} - 50512q^{46} - 47204q^{45} \\
& - 43891q^{44} - 40677q^{43} - 37517q^{42} - 34474q^{41} - 31522q^{40} - 28729q^{39} - 26035q^{38} \\
& - 23514q^{37} - 21128q^{36} - 18908q^{35} - 16826q^{34} - 14925q^{33} - 13152q^{32} - 11549q^{31} \\
& - 10081q^{30} - 8759q^{29} - 7563q^{28} - 6507q^{27} - 5551q^{26} - 4719q^{25} - 3984q^{24} - 3345q^{23} \\
& - 2784q^{22} - 2311q^{21} - 1896q^{20} - 1550q^{19} - 1255q^{18} - 1008q^{17} - 801q^{16} - 636q^{15} - 494q^{14} \\
& - 383q^{13} - 293q^{12} - 221q^{11} - 164q^{10} - 122q^9 - 88q^8 - 62q^7 - 43q^6 - 29q^5 - 19q^4 \\
& - 13q^3 - 7q^2 - 4q - 3 - \frac{1}{q} \\
f_{95}(q) = & 2q^{136} + 2q^{135} + 6q^{134} + 8q^{133} + 14q^{132} + 20q^{131} + 35q^{130} + 49q^{129} + 76q^{128} + 105q^{127} \\
& + 156q^{126} + 206q^{125} + 289q^{124} + 379q^{123} + 515q^{122} + 672q^{121} + 887q^{120} + 1138q^{119}
\end{aligned}$$

$$\begin{aligned}
& + 1475q^{118} + 1860q^{117} + 2365q^{116} + 2946q^{115} + 3685q^{114} + 4531q^{113} + 5591q^{112} \\
& + 6799q^{111} + 8287q^{110} + 9977q^{109} + 12021q^{108} + 14342q^{107} + 17123q^{106} + 20257q^{105} \\
& + 23972q^{104} + 28151q^{103} + 33050q^{102} + 38548q^{101} + 44941q^{100} + 52085q^{99} + 60337q^{98} \\
& + 69525q^{97} + 80055q^{96} + 91750q^{95} + 105073q^{94} + 119793q^{93} + 136462q^{92} + 154833q^{91} \\
& + 175489q^{90} + 198171q^{89} + 223526q^{88} + 251247q^{87} + 282067q^{86} + 315613q^{85} + 352682q^{84} \\
& + 392876q^{83} + 437042q^{82} + 484702q^{81} + 536796q^{80} + 592760q^{79} + 653584q^{78} + 718641q^{77} \\
& + 788970q^{76} + 863838q^{75} + 944364q^{74} + 1029680q^{73} + 1120951q^{72} + 1217232q^{71} \\
& + 1319695q^{70} + 1427250q^{69} + 1541148q^{68} + 1660134q^{67} + 1785484q^{66} + 1915810q^{65} \\
& + 2052400q^{64} + 2193702q^{63} + 2341053q^{62} + 2492696q^{61} + 2649991q^{60} + 2811050q^{59} \\
& + 2977212q^{58} + 3146405q^{57} + 3320028q^{56} + 3495803q^{55} + 3675148q^{54} + 3855646q^{53} \\
& + 4038708q^{52} + 4221770q^{51} + 4406293q^{50} + 4589527q^{49} + 4772986q^{48} + 4953828q^{47} \\
& + 5133575q^{46} + 5309264q^{45} + 5482517q^{44} + 5650256q^{43} + 5814175q^{42} + 5971158q^{41} \\
& + 6122947q^{40} + 6266410q^{39} + 6403409q^{38} + 6530749q^{37} + 6650426q^{36} + 6759292q^{35} \\
& + 6859416q^{34} + 6947700q^{33} + 7026370q^{32} + 7092358q^{31} + 7148031q^{30} + 7190426q^{29} \\
& + 7222011q^{28} + 7239947q^{27} + 7246857q^{26} + 7239947q^{25} + 7222011q^{24} + 7190426q^{23} \\
& + 7148031q^{22} + 7092358q^{21} + 7026370q^{20} + 6947700q^{19} + 6859416q^{18} + 6759292q^{17} \\
& + 6650426q^{16} + 6530749q^{15} + 6403409q^{14} + 6266410q^{13} + 6122947q^{12} + 5971158q^{11} \\
& + 5814175q^{10} + 5650256q^9 + 5482517q^8 + 5309264q^7 + 5133575q^6 + 4953828q^5 \\
& + 4772986q^4 + 4589527q^3 + 4406293q^2 + 4221770q + 4038708 + \frac{3855646}{q} + \frac{3675148}{q^2} \\
& + \frac{3495803}{q^3} + \frac{3320028}{q^4} + \frac{3146405}{q^5} + \frac{2977211}{q^6} + \frac{2811047}{q^7} + \frac{2649987}{q^8} + \frac{2492689}{q^9} \\
& + \frac{2341040}{q^{10}} + \frac{2193683}{q^{11}} + \frac{2052371}{q^{12}} + \frac{1915769}{q^{13}} + \frac{1785426}{q^{14}} + \frac{1660054}{q^{15}} + \frac{1541040}{q^{16}} \\
& + \frac{1427108}{q^{17}} + \frac{1319509}{q^{18}} + \frac{1216997}{q^{19}} + \frac{1120655}{q^{20}} + \frac{1029313}{q^{21}} + \frac{943912}{q^{22}} + \frac{863295}{q^{23}} + \frac{788318}{q^{24}} \\
& + \frac{717874}{q^{25}} + \frac{652685}{q^{26}} + \frac{591724}{q^{27}} + \frac{535609}{q^{28}} + \frac{483363}{q^{29}} + \frac{435536}{q^{30}} + \frac{391207}{q^{31}} + \frac{350843}{q^{32}} \\
& + \frac{313613}{q^{33}} + \frac{279905}{q^{34}} + \frac{248940}{q^{35}} + \frac{221077}{q^{36}} + \frac{195604}{q^{37}} + \frac{172813}{q^{38}} + \frac{152077}{q^{39}} + \frac{133640}{q^{40}} \\
& + \frac{116937}{q^{41}} + \frac{102194}{q^{42}} + \frac{88894}{q^{43}} + \frac{77233}{q^{44}} + \frac{66769}{q^{45}} + \frac{57661}{q^{46}} + \frac{49518}{q^{47}} + \frac{42492}{q^{48}} + \frac{36241}{q^{49}} \\
& + \frac{30888}{q^{50}} + \frac{26151}{q^{51}} + \frac{22133}{q^{52}} + \frac{18588}{q^{53}} + \frac{15617}{q^{54}} + \frac{13003}{q^{55}} + \frac{10834}{q^{56}} + \frac{8941}{q^{57}} + \frac{7388}{q^{58}} + \frac{6032}{q^{59}} \\
& + \frac{4939}{q^{60}} + \frac{3988}{q^{61}} + \frac{3233}{q^{62}} + \frac{2579}{q^{63}} + \frac{2069}{q^{64}} + \frac{1625}{q^{65}} + \frac{1289}{q^{66}} + \frac{996}{q^{67}} + \frac{779}{q^{68}} + \frac{592}{q^{69}} + \frac{457}{q^{70}} + \frac{338}{q^{71}} \\
& + \frac{258}{q^{72}} + \frac{185}{q^{73}} + \frac{138}{q^{74}} + \frac{96}{q^{75}} + \frac{70}{q^{76}} + \frac{46}{q^{77}} + \frac{34}{q^{78}} + \frac{20}{q^{79}} + \frac{14}{q^{80}} + \frac{8}{q^{81}} + \frac{6}{q^{82}} + \frac{2}{q^{83}} + \frac{2}{q^{84}} \\
f_{97}(q) = & - 2q^{138} - 2q^{137} - 6q^{136} - 8q^{135} - 15q^{134} - 23q^{133} - 38q^{132} - 53q^{131} - 83q^{130} - 112q^{129}
\end{aligned}$$

$$\begin{aligned}
& -159q^{128} - 211q^{127} - 290q^{126} - 372q^{125} - 492q^{124} - 621q^{123} - 795q^{122} - 986q^{121} \\
& -1237q^{120} - 1509q^{119} - 1870q^{118} - 2256q^{117} - 2747q^{116} - 3291q^{115} - 3968q^{114} - 4708q^{113} \\
& -5618q^{112} - 6618q^{111} - 7815q^{110} - 9126q^{109} - 10683q^{108} - 12365q^{107} - 14337q^{106} \\
& -16460q^{105} - 18898q^{104} - 21518q^{103} - 24498q^{102} - 27655q^{101} - 31208q^{100} - 34961q^{99} \\
& -39122q^{98} - 43481q^{97} - 48283q^{96} - 53251q^{95} - 58671q^{94} - 64247q^{93} - 70248q^{92} \\
& -76369q^{91} - 82909q^{90} - 89489q^{89} - 96453q^{88} - 103408q^{87} - 110671q^{86} - 117835q^{85} \\
& -125260q^{84} - 132470q^{83} - 139865q^{82} - 146953q^{81} - 154109q^{80} - 160849q^{79} - 167589q^{78} \\
& -173771q^{77} - 179860q^{76} - 185309q^{75} - 190550q^{74} - 195053q^{73} - 199295q^{72} - 202693q^{71} \\
& -205766q^{70} - 207955q^{69} - 209750q^{68} - 210625q^{67} - 211113q^{66} - 210625q^{65} - 209750q^{64} \\
& -207955q^{63} - 205766q^{62} - 202693q^{61} - 199295q^{60} - 195053q^{59} - 190550q^{58} - 185309q^{57} \\
& -179860q^{56} - 173771q^{55} - 167589q^{54} - 160849q^{53} - 154109q^{52} - 146953q^{51} - 139865q^{50} \\
& -132470q^{49} - 125260q^{48} - 117835q^{47} - 110671q^{46} - 103408q^{45} - 96453q^{44} - 89489q^{43} \\
& -82909q^{42} - 76369q^{41} - 70248q^{40} - 64247q^{39} - 58671q^{38} - 53251q^{37} - 48283q^{36} \\
& -43481q^{35} - 39122q^{34} - 34961q^{33} - 31208q^{32} - 27655q^{31} - 24497q^{30} - 21515q^{29} \\
& -18894q^{28} - 16453q^{27} - 14324q^{26} - 12348q^{25} - 10658q^{24} - 9093q^{23} - 7772q^{22} - 6564q^{21} \\
& -5551q^{20} - 4631q^{19} - 3880q^{18} - 3194q^{17} - 2643q^{16} - 2148q^{15} - 1755q^{14} - 1401q^{13} \\
& -1133q^{12} - 889q^{11} - 707q^{10} - 544q^9 - 425q^8 - 318q^7 - 247q^6 - 178q^5 - 134q^4 - 95q^3 \\
& -70q^2 - 46q - 34 - \frac{20}{q} - \frac{14}{q^2} - \frac{8}{q^3} - \frac{6}{q^4} - \frac{2}{q^5} - \frac{2}{q^6}.
\end{aligned}$$

Using the recursion relation (9) in [1] and the above initial data, we obtain, for example,  $f_{99}$  and  $f_{101}$ .

$$\begin{aligned}
f_{99}(q) = & q^{148} + 3q^{147} + 4q^{146} + 7q^{145} + 13q^{144} + 19q^{143} + 29q^{142} + 45q^{141} + 64q^{140} + 97q^{139} \\
& + 137q^{138} + 192q^{137} + 262q^{136} + 363q^{135} + 475q^{134} + 632q^{133} + 828q^{132} + 1079q^{131} \\
& + 1385q^{130} + 1785q^{129} + 2257q^{128} + 2859q^{127} + 3574q^{126} + 4454q^{125} + 5499q^{124} \\
& + 6782q^{123} + 8269q^{122} + 10076q^{121} + 12182q^{120} + 14689q^{119} + 17588q^{118} + 21024q^{117} \\
& + 24957q^{116} + 29578q^{115} + 34862q^{114} + 40991q^{113} + 47977q^{112} + 56047q^{111} + 65162q^{110} \\
& + 75627q^{109} + 87436q^{108} + 100875q^{107} + 115973q^{106} + 133090q^{105} + 152223q^{104} \\
& + 173796q^{103} + 197846q^{102} + 224787q^{101} + 254715q^{100} + 288123q^{99} + 325026q^{98} \\
& + 366027q^{97} + 411206q^{96} + 461113q^{95} + 515887q^{94} + 576158q^{93} + 642003q^{92} + 714125q^{91} \\
& + 792633q^{90} + 878190q^{89} + 970956q^{88} + 1071647q^{87} + 1180302q^{86} + 1297720q^{85} \\
& + 1423977q^{84} + 1559750q^{83} + 1705123q^{82} + 1860827q^{81} + 2026797q^{80} + 2203794q^{79} \\
& + 2391721q^{78} + 2591201q^{77} + 2802128q^{76} + 3025118q^{75} + 3259834q^{74} + 3506904q^{73} \\
& + 3765949q^{72} + 4037374q^{71} + 4320724q^{70} + 4616400q^{69} + 4923670q^{68} + 5242901q^{67} \\
& + 5573242q^{66} + 5914833q^{65} + 6266753q^{64} + 6629069q^{63} + 7000524q^{62} + 7381167q^{61} \\
& + 7769650q^{60} + 8165746q^{59} + 8567991q^{58} + 8976142q^{57} + 9388421q^{56} + 9804559q^{55}
\end{aligned}$$

$$\begin{aligned}
& + 10222689q^{54} + 10642306q^{53} + 11061511q^{52} + 11479791q^{51} + 11894949q^{50} + 12306545q^{49} \\
& + 12712390q^{48} + 13111827q^{47} + 13502683q^{46} + 13884422q^{45} + 14254688q^{44} + 14613062q^{43} \\
& + 14957266q^{42} + 15286787q^{41} + 15599512q^{40} + 15895110q^{39} + 16171340q^{38} + 16428123q^{37} \\
& + 16663441q^{36} + 16877174q^{35} + 17067534q^{34} + 17234699q^{33} + 17376881q^{32} + 17494540q^{31} \\
& + 17586169q^{30} + 17652279q^{29} + 17691688q^{28} + 17705222q^{27} + 17691688q^{26} + 17652279q^{25} \\
& + 17586169q^{24} + 17494540q^{23} + 17376881q^{22} + 17234699q^{21} + 17067534q^{20} + 16877174q^{19} \\
& + 16663441q^{18} + 16428123q^{17} + 16171340q^{16} + 15895110q^{15} + 15599512q^{14} + 15286787q^{13} \\
& + 14957266q^{12} + 14613062q^{11} + 14254688q^{10} + 13884422q^9 + 13502683q^8 + 13111827q^7 \\
& + 12712390q^6 + 12306545q^5 + 11894949q^4 + 11479791q^3 + 11061511q^2 + 10642306q \\
& + 10222689 + \frac{9804559}{q} + \frac{9388421}{q^2} + \frac{8976140}{q^3} + \frac{8567989}{q^4} + \frac{8165740}{q^5} + \frac{7769642}{q^6} \\
& + \frac{7381153}{q^7} + \frac{7000504}{q^8} + \frac{6629035}{q^9} + \frac{6266708}{q^{10}} + \frac{5914767}{q^{11}} + \frac{5573154}{q^{12}} + \frac{5242778}{q^{13}} \\
& + \frac{4923512}{q^{14}} + \frac{4616185}{q^{15}} + \frac{4320456}{q^{16}} + \frac{4037025}{q^{17}} + \frac{3765518}{q^{18}} + \frac{3506363}{q^{19}} + \frac{3259179}{q^{20}} \\
& + \frac{3024311}{q^{21}} + \frac{2801174}{q^{22}} + \frac{2590053}{q^{23}} + \frac{2390380}{q^{24}} + \frac{2202215}{q^{25}} + \frac{2024987}{q^{26}} + \frac{1858731}{q^{27}} \\
& + \frac{1702760}{q^{28}} + \frac{1557064}{q^{29}} + \frac{1420988}{q^{30}} + \frac{1294384}{q^{31}} + \frac{1176647}{q^{32}} + \frac{1067621}{q^{33}} + \frac{966613}{q^{34}} \\
& + \frac{873484}{q^{35}} + \frac{787622}{q^{36}} + \frac{708780}{q^{37}} + \frac{636395}{q^{38}} + \frac{570257}{q^{39}} + \frac{509784}{q^{40}} + \frac{454786}{q^{41}} + \frac{404747}{q^{42}} \\
& + \frac{359428}{q^{43}} + \frac{318385}{q^{44}} + \frac{281421}{q^{45}} + \frac{248074}{q^{46}} + \frac{218188}{q^{47}} + \frac{191387}{q^{48}} + \frac{167469}{q^{49}} + \frac{146120}{q^{50}} \\
& + \frac{127189}{q^{51}} + \frac{110365}{q^{52}} + \frac{95530}{q^{53}} + \frac{82425}{q^{54}} + \frac{70921}{q^{55}} + \frac{60819}{q^{56}} + \frac{52021}{q^{57}} + \frac{44322}{q^{58}} + \frac{37655}{q^{59}} \\
& + \frac{31873}{q^{60}} + \frac{26892}{q^{61}} + \frac{22594}{q^{62}} + \frac{18928}{q^{63}} + \frac{15778}{q^{64}} + \frac{13110}{q^{65}} + \frac{10841}{q^{66}} + \frac{8928}{q^{67}} + \frac{7315}{q^{68}} + \frac{5975}{q^{69}} \\
& + \frac{4844}{q^{70}} + \frac{3913}{q^{71}} + \frac{3143}{q^{72}} + \frac{2510}{q^{73}} + \frac{1989}{q^{74}} + \frac{1570}{q^{75}} + \frac{1227}{q^{76}} + \frac{955}{q^{77}} + \frac{737}{q^{78}} + \frac{562}{q^{79}} + \frac{425}{q^{80}} + \frac{321}{q^{81}} \\
& + \frac{237}{q^{82}} + \frac{174}{q^{83}} + \frac{126}{q^{84}} + \frac{90}{q^{85}} + \frac{62}{q^{86}} + \frac{43}{q^{87}} + \frac{29}{q^{88}} + \frac{19}{q^{89}} + \frac{13}{q^{90}} + \frac{7}{q^{91}} + \frac{4}{q^{92}} + \frac{3}{q^{93}} + \frac{1}{q^{94}} \\
f_{101}(q) = & -q^{150} - 3q^{149} - 4q^{148} - 7q^{147} - 13q^{146} - 22q^{145} - 31q^{144} - 49q^{143} - 70q^{142} - 104q^{141} \\
& - 143q^{140} - 200q^{139} - 267q^{138} - 362q^{137} - 469q^{136} - 615q^{135} - 785q^{134} - 1004q^{133} \\
& - 1255q^{132} - 1572q^{131} - 1934q^{130} - 2385q^{129} - 2896q^{128} - 3518q^{127} - 4232q^{126} \\
& - 5092q^{125} - 6058q^{124} - 7209q^{123} - 8518q^{122} - 10050q^{121} - 11783q^{120} - 13792q^{119} \\
& - 16049q^{118} - 18640q^{117} - 21530q^{116} - 24809q^{115} - 28458q^{114} - 32550q^{113} - 37056q^{112} \\
& - 42074q^{111} - 47562q^{110} - 53611q^{109} - 60179q^{108} - 67353q^{107} - 75086q^{106} - 83471q^{105} \\
& - 92432q^{104} - 102059q^{103} - 112288q^{102} - 123190q^{101} - 134666q^{100} - 146812q^{99} \\
& - 159497q^{98} - 172808q^{97} - 186601q^{96} - 200949q^{95} - 215696q^{94} - 230912q^{93}
\end{aligned}$$

$$\begin{aligned}
& -246398q^{92} - 262233q^{91} - 278215q^{90} - 294397q^{89} - 310547q^{88} - 326745q^{87} \\
& - 342737q^{86} - 358588q^{85} - 374042q^{84} - 389156q^{83} - 403679q^{82} - 417684q^{81} \\
& - 430885q^{80} - 443382q^{79} - 454907q^{78} - 465550q^{77} - 475049q^{76} - 483527q^{75} \\
& - 490725q^{74} - 496781q^{73} - 501455q^{72} - 504899q^{71} - 506903q^{70} - 507651q^{69} \\
& - 506903q^{68} - 504899q^{67} - 501455q^{66} - 496781q^{65} - 490725q^{64} - 483527q^{63} \\
& - 475049q^{62} - 465550q^{61} - 454907q^{60} - 443382q^{59} - 430885q^{58} - 417684q^{57} \\
& - 403679q^{56} - 389156q^{55} - 374042q^{54} - 358588q^{53} - 342737q^{52} - 326745q^{51} \\
& - 310547q^{50} - 294397q^{49} - 278215q^{48} - 262233q^{47} - 246398q^{46} - 230912q^{45} \\
& - 215696q^{44} - 200949q^{43} - 186601q^{42} - 172808q^{41} - 159497q^{40} - 146812q^{39} \\
& - 134666q^{38} - 123190q^{37} - 112288q^{36} - 102059q^{35} - 92432q^{34} - 83469q^{33} - 75084q^{32} \\
& - 67347q^{31} - 60171q^{30} - 53597q^{29} - 47543q^{28} - 42044q^{27} - 37018q^{26} - 32495q^{25} \\
& - 28392q^{24} - 24722q^{23} - 21428q^{22} - 18511q^{21} - 15904q^{20} - 13620q^{19} - 11597q^{18} \\
& - 9840q^{17} - 8299q^{16} - 6972q^{15} - 5820q^{14} - 4841q^{13} - 3994q^{12} - 3281q^{11} - 2677q^{10} \\
& - 2175q^9 - 1748q^8 - 1400q^7 - 1110q^6 - 875q^5 - 683q^4 - 528q^3 - 403q^2 - 307q - 229 \\
& - \frac{170}{q} - \frac{124}{q^2} - \frac{90}{q^3} - \frac{62}{q^4} - \frac{43}{q^5} - \frac{29}{q^6} - \frac{19}{q^7} - \frac{13}{q^8} - \frac{7}{q^9} - \frac{4}{q^{10}} - \frac{3}{q^{11}} - \frac{1}{q^{12}}.
\end{aligned}$$

## References

- [1] Chae J., A Cable Knot and BPS Series, arXiv (January 2021)
